# Supplementary material for: ReFineVLA: Multimodal Reasoning-Aware Generalist Robotic Policies via Teacher-Guided Fine-Tuning
Source: arXiv:2604.17800 source file (2026-04-20)
Supplement: Supplementary file 1 [file libero.tex]

\subsection{Additional Experimental Results on LIBERO Simulation Benchmark}

\begin{figure}[h!]
    \centering
    \begin{subfigure}[b]{0.22\textwidth}
        \includegraphics[width=\textwidth]{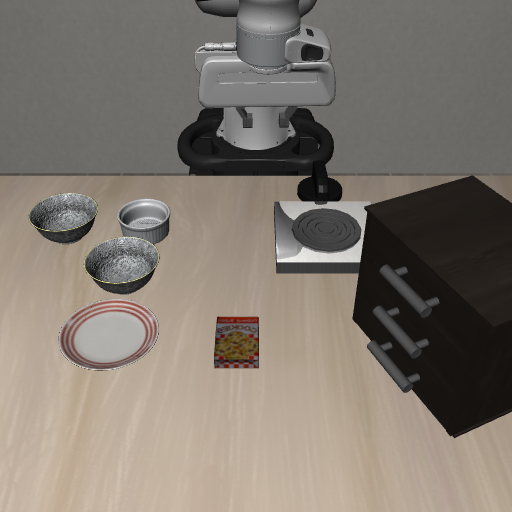}
        \caption{LIBERO-Spatial}
    \end{subfigure}
    \hfill
    \begin{subfigure}[b]{0.22\textwidth}
        \includegraphics[width=\textwidth]{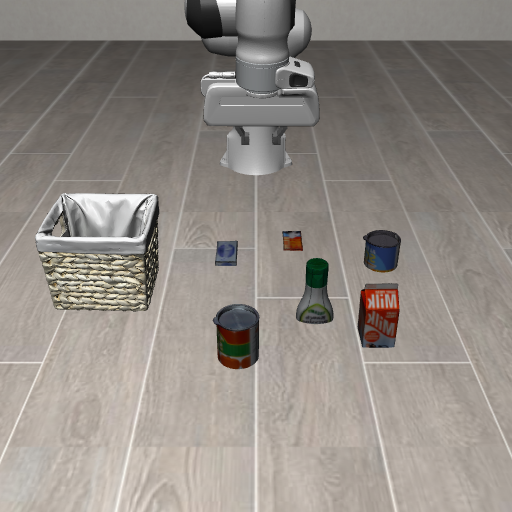}
        \caption{LIBERO-Object}
    \end{subfigure}
    \hfill
    \begin{subfigure}[b]{0.22\textwidth}
        \includegraphics[width=\textwidth]{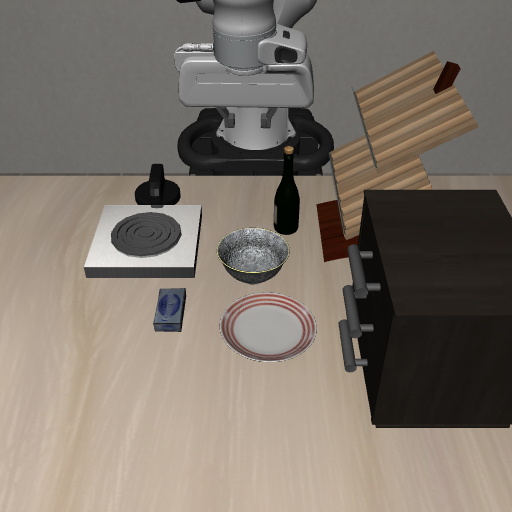}
        \caption{LIBERO-Goal}
    \end{subfigure}
    \hfill
    \begin{subfigure}[b]{0.22\textwidth}
        \includegraphics[width=\textwidth]{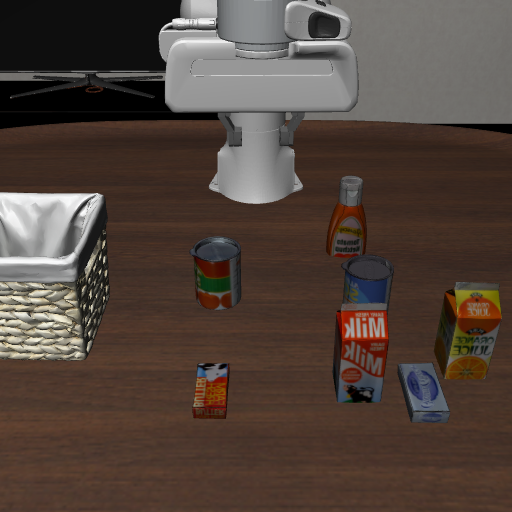}
        \caption{LIBERO-Long}
    \end{subfigure}
    \vspace{-3pt}
    \caption{Four test suites in the LIBERO simulation benchmark, including \textbf{(a)} LIBERO-Spatial, \textbf{(b)} LIBERO-Object, \textbf{(c)} LIBERO-Goal, and \textbf{(d)} LIBERO-Long.}
    \label{fig:libero_test_suites}
    \vspace{-4pt}
\end{figure}

In addition to SimplerEnv and WIDOWX-$250$ real robot experiments, we report additional experiments on the LIBERO simulation benchmark. In specific, we take the four suites from LIBERO: \textbf{LIBERO-long}, \textbf{LIBERO-Spatial}, \textbf{LIBERO-Object}, \textbf{LIBERO-Goal}, each with $10$ tasks and $50$ human tele-operated demonstrations, and evaluate the multitask performance of the pre-trained VLA-based policy. The test suites as shown in Figure \ref{fig:libero_test_suites} are:
\begin{itemize}
    \vspace{-4pt}
    \item \textbf{LIBERO-Spatial}: Contains the same set of objects but in varying layouts, testing the model’s ability to understand spatial relationships. Example language instruction: ``\textit{pick up the black bowl between the plate and the ramekin and place it on the plate}''.
    \vspace{-4pt}
    \item \textbf{LIBERO-Object}: Features consistent scene layouts but introduces different objects, evaluating the model’s understanding of object types. Example language instruction: \textit{pick up the alphabet soup and place it in the basket}.
    \item \textbf{LIBERO-Goal}: Maintains the same objects and layouts while varying task goals, assessing the model’s knowledge of diverse task-oriented behaviors. Example language instruction: ``\textit{put both the alphabet soup and the tomato sauce in the basket}''.
    \vspace{-4pt}
    \item \textbf{LIBERO-Long} (also referred to as \textbf{LIBERO-10}): Comprises long-horizon tasks involving diverse objects, layouts, and task goals, challenging the model's ability to handle extended planning and execution. Example language instruction: ``\textit{open the middle drawer of the cabinet}''.
    \vspace{-4pt}
\end{itemize}

\begin{table}[h]
    \vspace{-4pt}
    \centering
    \resizebox{\textwidth}{!}{
    \begin{tabular}{lcccc c}
        \midrule
        \textbf{Method} & \textbf{LIBERO-Spatial} & \textbf{LIBERO-Object} & \textbf{LIBERO-Goal} & \textbf{LIBERO-Long} & \textbf{Average} \\ 
        \midrule
        \textbf{TraceVLA fine-tuned} & $\mathbf{84.6\% \pm 0.2\%}$ & $\mathbf{85.2\% \pm 0.4\%}$ & $\mathbf{75.1\% \pm 0.3\%}$ & $\mathbf{54.1\% \pm 1.0\%}$ & $\mathbf{74.8\% \pm 0.4\%}$ \\
        OpenVLA fine-tuned & $82.6\% \pm 0.4\%$ & $83.8\% \pm 0.6\%$ & $70.4\% \pm 0.5\%$ & $45.7\% \pm 0.6\%$ & $70.6\% \pm 0.4\%$ \\ 
        \midrule
        \end{tabular}
    }
    \vspace{-4pt}
    \caption{Multitask success rates on LIBERO-Spatial, LIBERO-Object, LIBERO-Goal, LIBERO-Long, and average performance across four test suites.}
    \label{tab:libero-results}
\end{table}

Following OpenVLA, we pre-process the data by filtering out non-successful trajectories and removing all steps with actions that have near-zero norms and do not change the gripper's status. 
For TraceVLA, we also annotate visual trace following the same procedure performed on BridgeData-v2 and Google Robot datasets. We then fine-tune both the OpenVLA model and the TraceVLA-7B model on the combined dataset from these four suites and report their multitask success rates on each suite in Table~\ref {tab:libero-results}. Compared to the results in OpenVLA, we only fine-tune a single model on the mixture of all four suites instead of fine-tuning each suite separately. For each task, we evaluate each method using three random seeds, perform $50$ rollouts for each seed with random initial states, and report the average performance across all $10$ tasks per suite. As shown in Table~\ref{tab:libero-results}, compared with OpenVLA, the superior performance of TraceVLA across each benchmark suite further demonstrates the benefits of our visual trace prompting.
