# Supplementary material for: ReFineVLA: Multimodal Reasoning-Aware Generalist Robotic Policies via Teacher-Guided Fine-Tuning
Source: arXiv:2604.17800 source file (2026-04-20)
Supplement: Supplementary file 2 [file table.tex]

% --- Define and Set Width Variables ---
% Set the column widths as fractions of \linewidth
% Adjust these fractions as needed.
% Ensure the sum of fractions is slightly less than 1.0 to leave space for \tabcolsep.
\setlength{\colAwidth}{0.25\linewidth}
\setlength{\colBwidth}{0.1\linewidth}
\setlength{\colCwidth}{0.7\linewidth}
\setlength{\figurewidth}{\colAwidth}

\begin{table}[H]
    \centering
    \small % Use smaller font size

    % Define the table structure:
    % Column 1: aligned center for images using \adjustbox
    % Column 2: aligned left, controlled by \minipage for captions
    \begin{tabular}{ll}
        \toprule % Top rule line

        % --- First Row: Fridge ---
        \adjustbox{valign=t}{\includegraphics[width=\figurewidth]{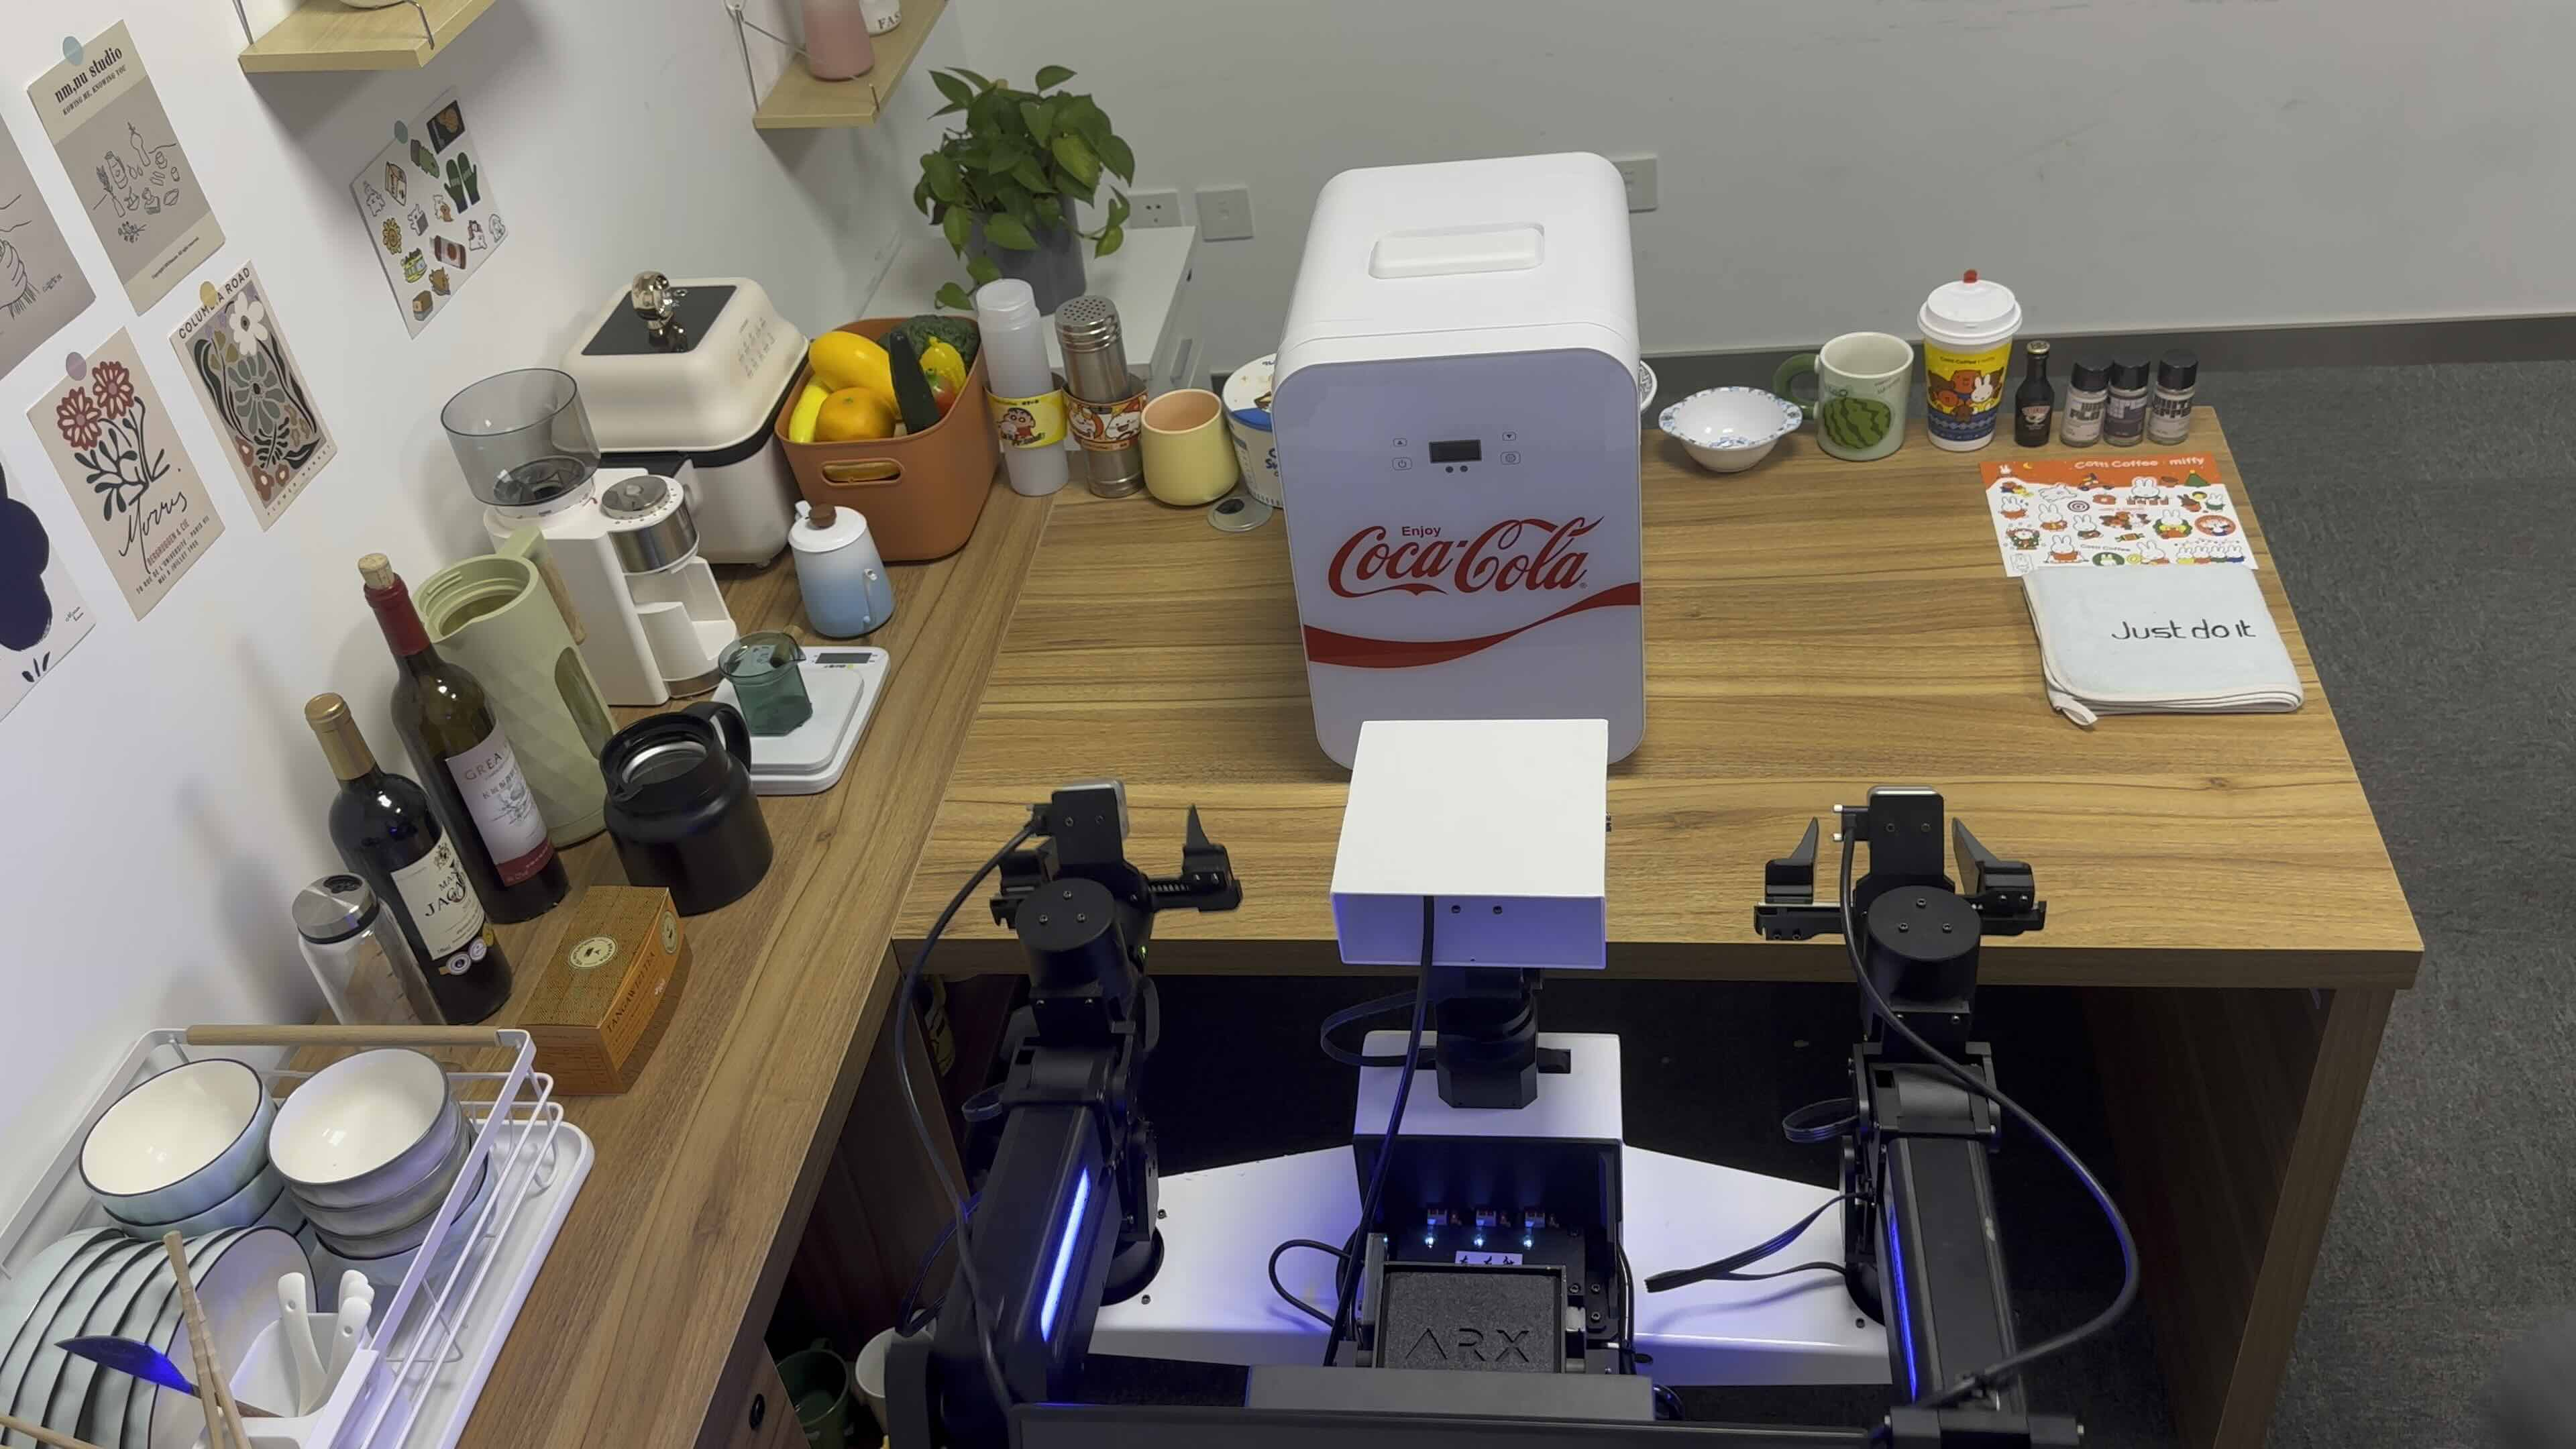}}
        & % Column separator
        \begin{minipage}[t]{\colCwidth}
            \raggedright
            \textbf{Instruction}: Give me an icy cola.\\
            \textbf{Reasoning}:\\
            \textsf{Scene description}: The cola is out of sight, maybe in the fridge. \\
            \textsf{Plan}:  1. Open the fridge door.  2. Pick up the icy cola bottle and place it on the table.  3. Close the fridge door.
        \end{minipage} \\ % End of table row
        \midrule % Mid rule line

        % --- Third Row: Occlusion ---
        \adjustbox{valign=t}{\includegraphics[width=\figurewidth]{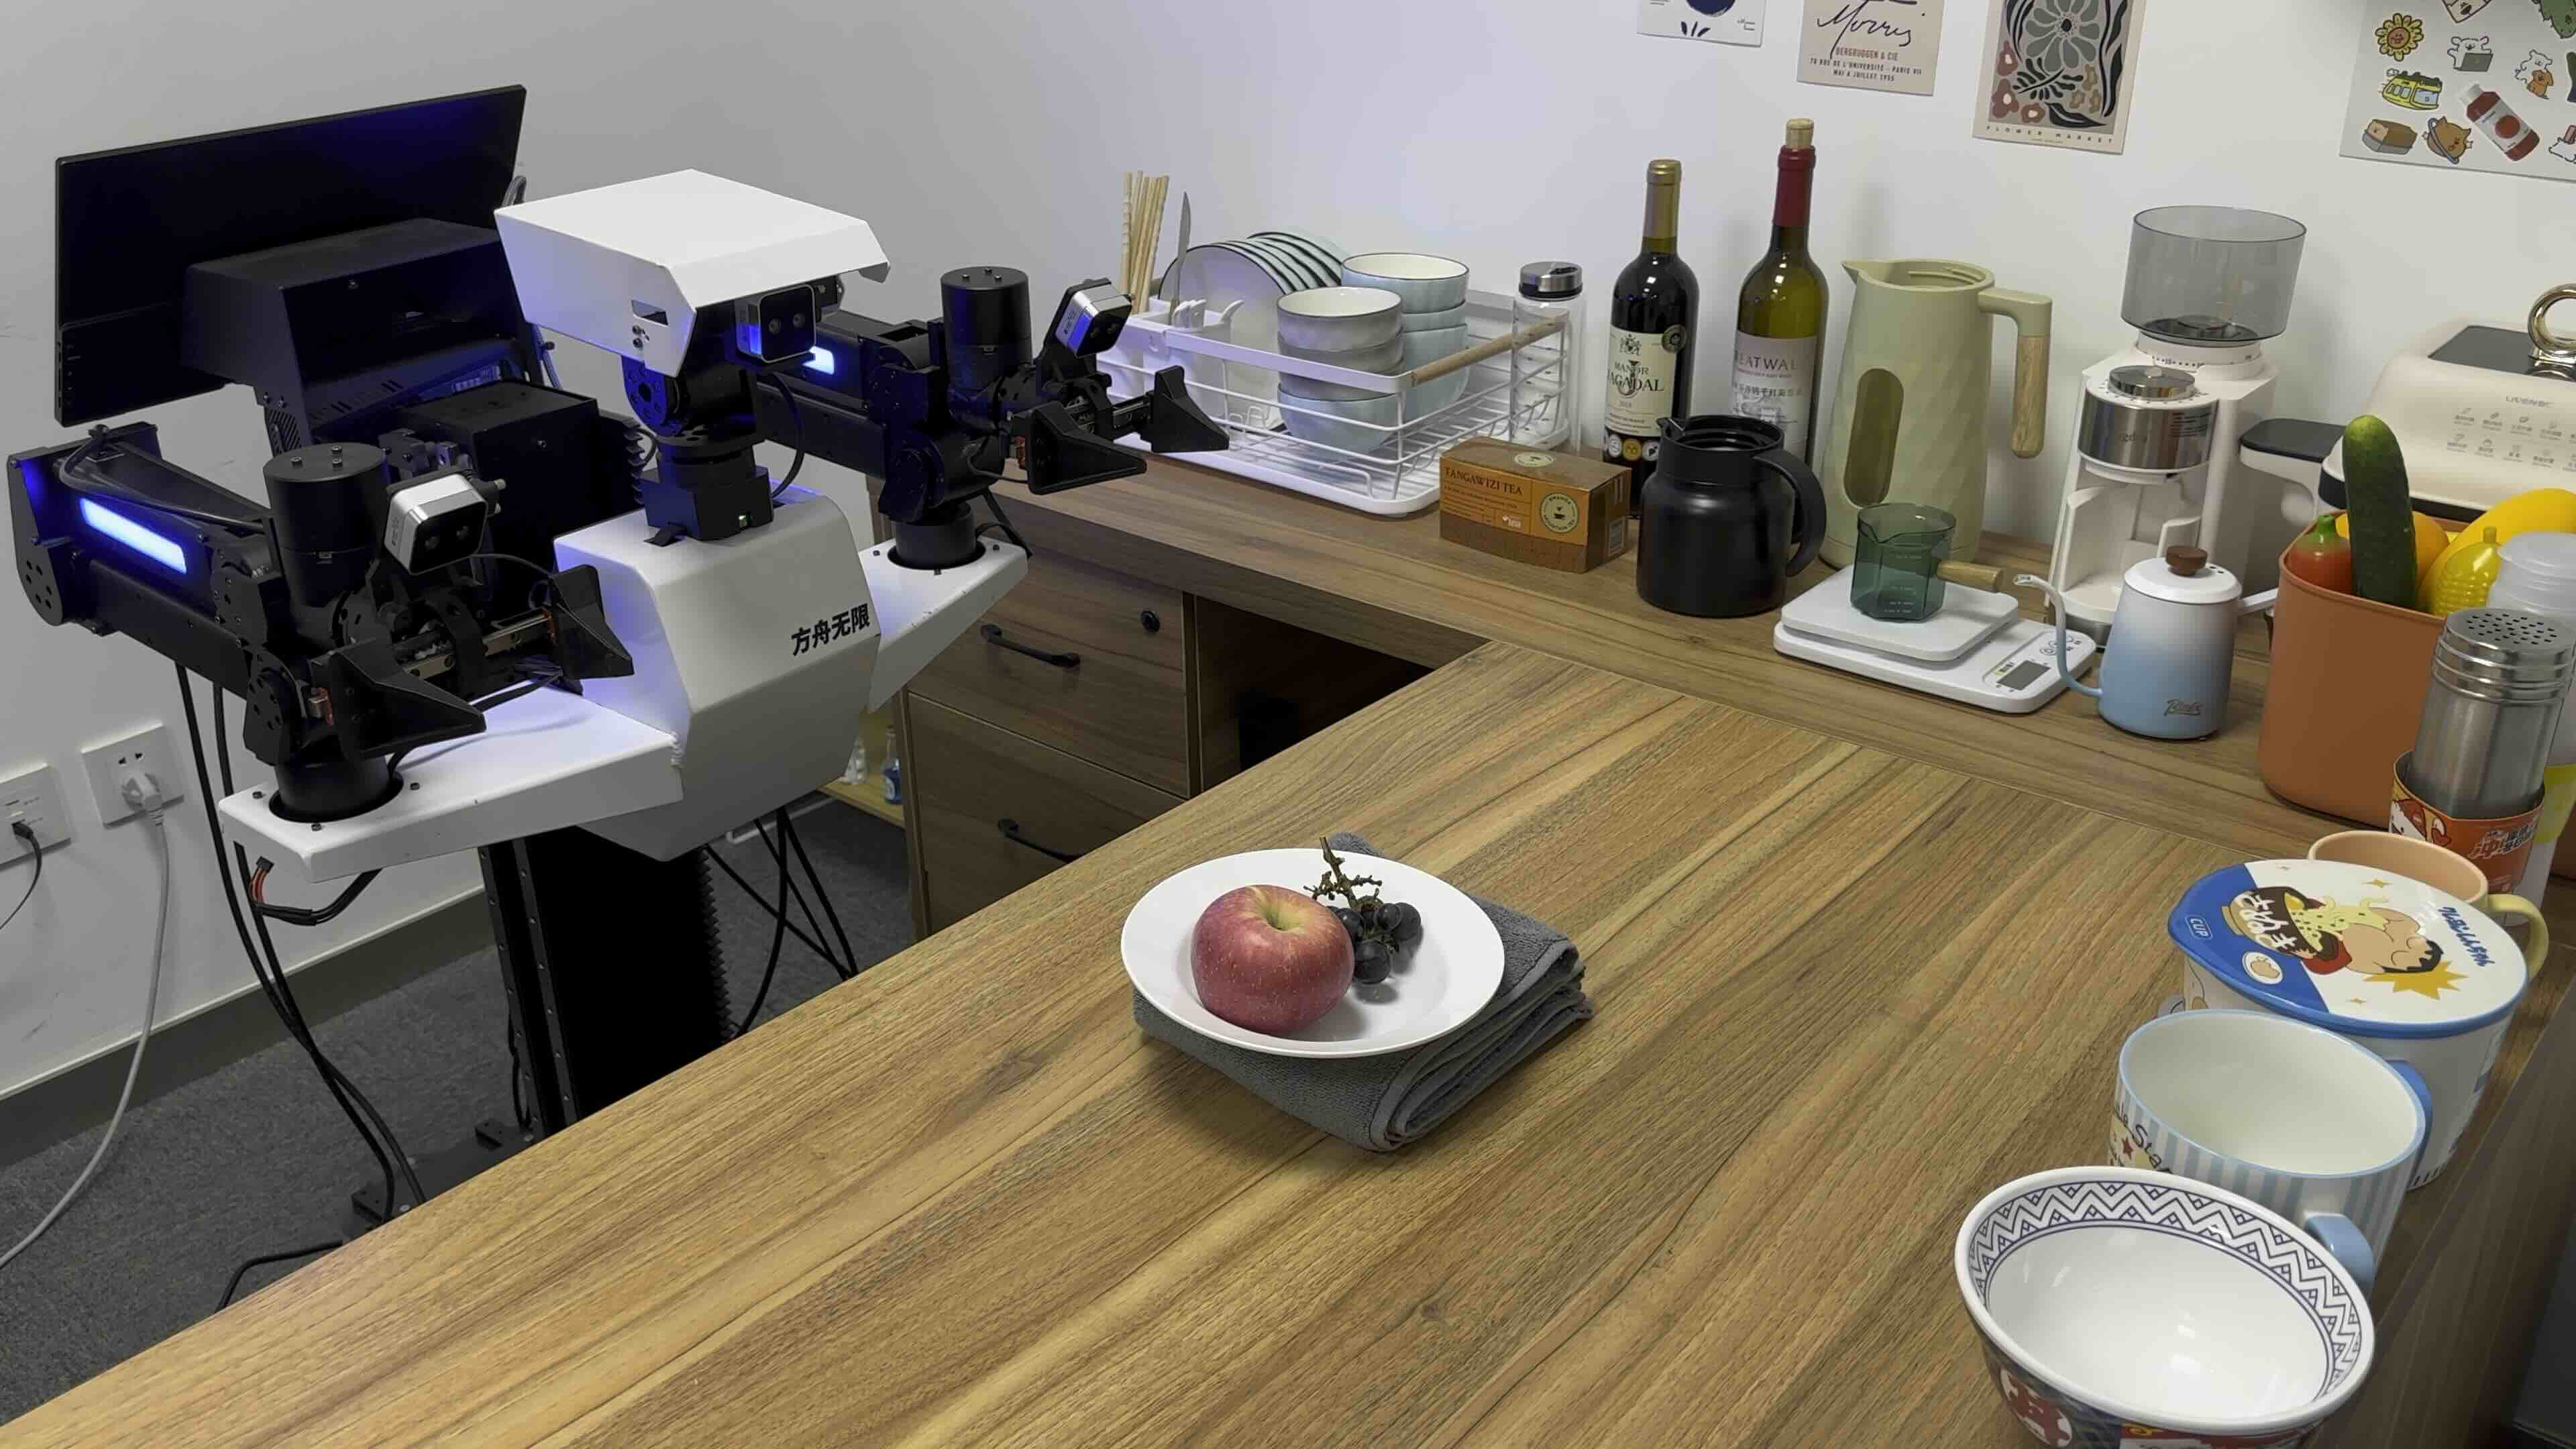}}
        & % Column separator
        \begin{minipage}[t]{\colCwidth}
            \raggedright
            \textbf{Instruction}: Pass me an empty plate. \\
            \textbf{Reasoning}:\\
            \textsf{Scene description}: The grapes and apple are on the plate. \\
            \textsf{Plan}:  1. Pick up the grapes and place them on the table.
            2. Pick up the apple and place it on the table.
            3. Pick up the empty plate.
        \end{minipage} \\ % End of table row
        \midrule % Mid rule line

        % --- Fifth Row: Drinks ---
        \adjustbox{valign=\imagevalign}{\includegraphics[width=\figurewidth]{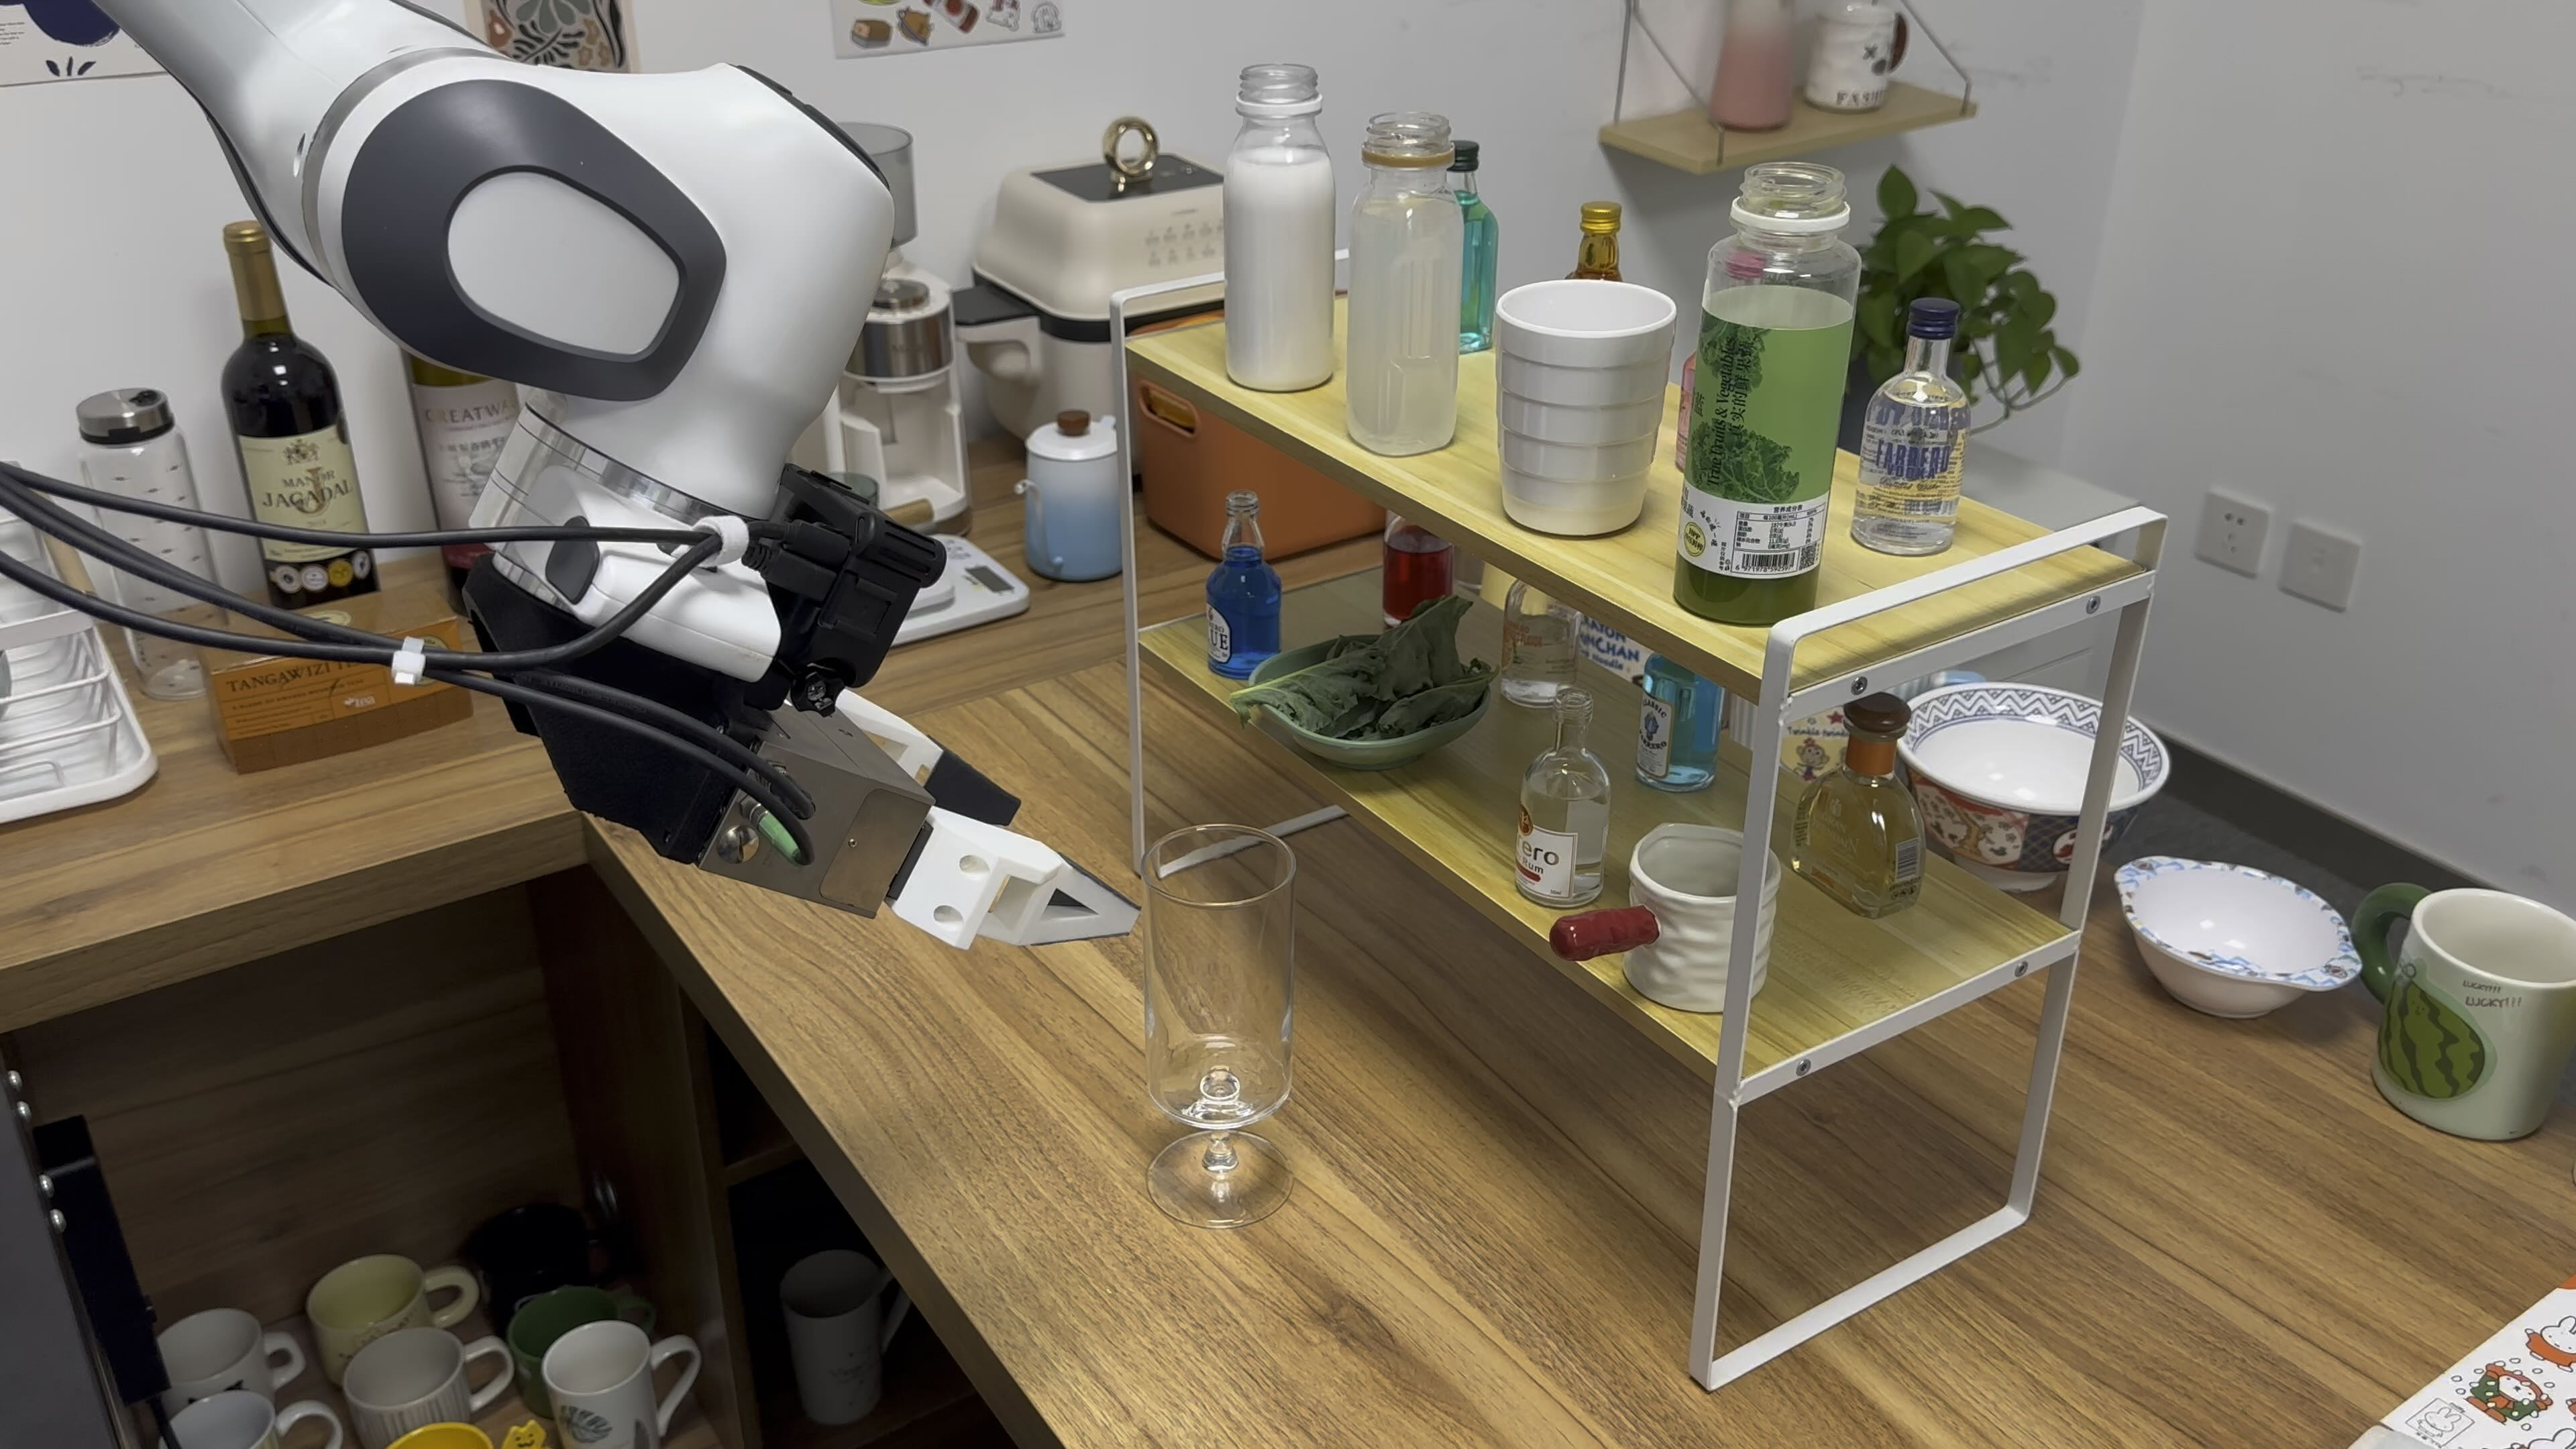}}
        & % Column separator
        \begin{minipage}[\imagevalign]{\colCwidth}
            \raggedright
            \textbf{Instruction}: I'm exhausted — can you make me a drink to keep me awake? \\
            \textbf{Reasoning}:\\
            I need to make a \texttt{coconut latte}. \\
            \textsf{Plan}:   
            1. Add thick coconut milk to the coffee cup.  
            2. Pour espresso into the cup.  
            3. Drop in ice cubes.
            \rule{\linewidth}{0.2pt} % Horizontal line
            \textbf{Instruction}: I've been eating clean and need a nutritious drink. \\
            \textbf{Reasoning}:\\
            I need to make a glass of \texttt{kale juice} with some kale leaves and ice cubes. \\
            \textsf{Plan}:   
            1. Pour kale juice into the cup.  
            2. Put a kale leaf in the cup.  
            3. Add ice cubes to the cup.
            \rule{\linewidth}{0.2pt} % Horizontal line
            \textbf{Instruction}: I'm feeling kind of down today. Can you fix me a drink? \\
            \textbf{Reasoning}:\\
            I need to make a \texttt{Blue Mood} cocktail. \\
            \textsf{Plan}:   
            1. Pour in white rum.  
            2. Add Blue Curacao.  
            3. Mix in lemon juice.  
            4. Drop in ice cubes. 
        \end{minipage} \\ % End of table row
        \midrule

        % --- Fourth Row: Tool ---
        \adjustbox{valign=t}{\includegraphics[width=\figurewidth]{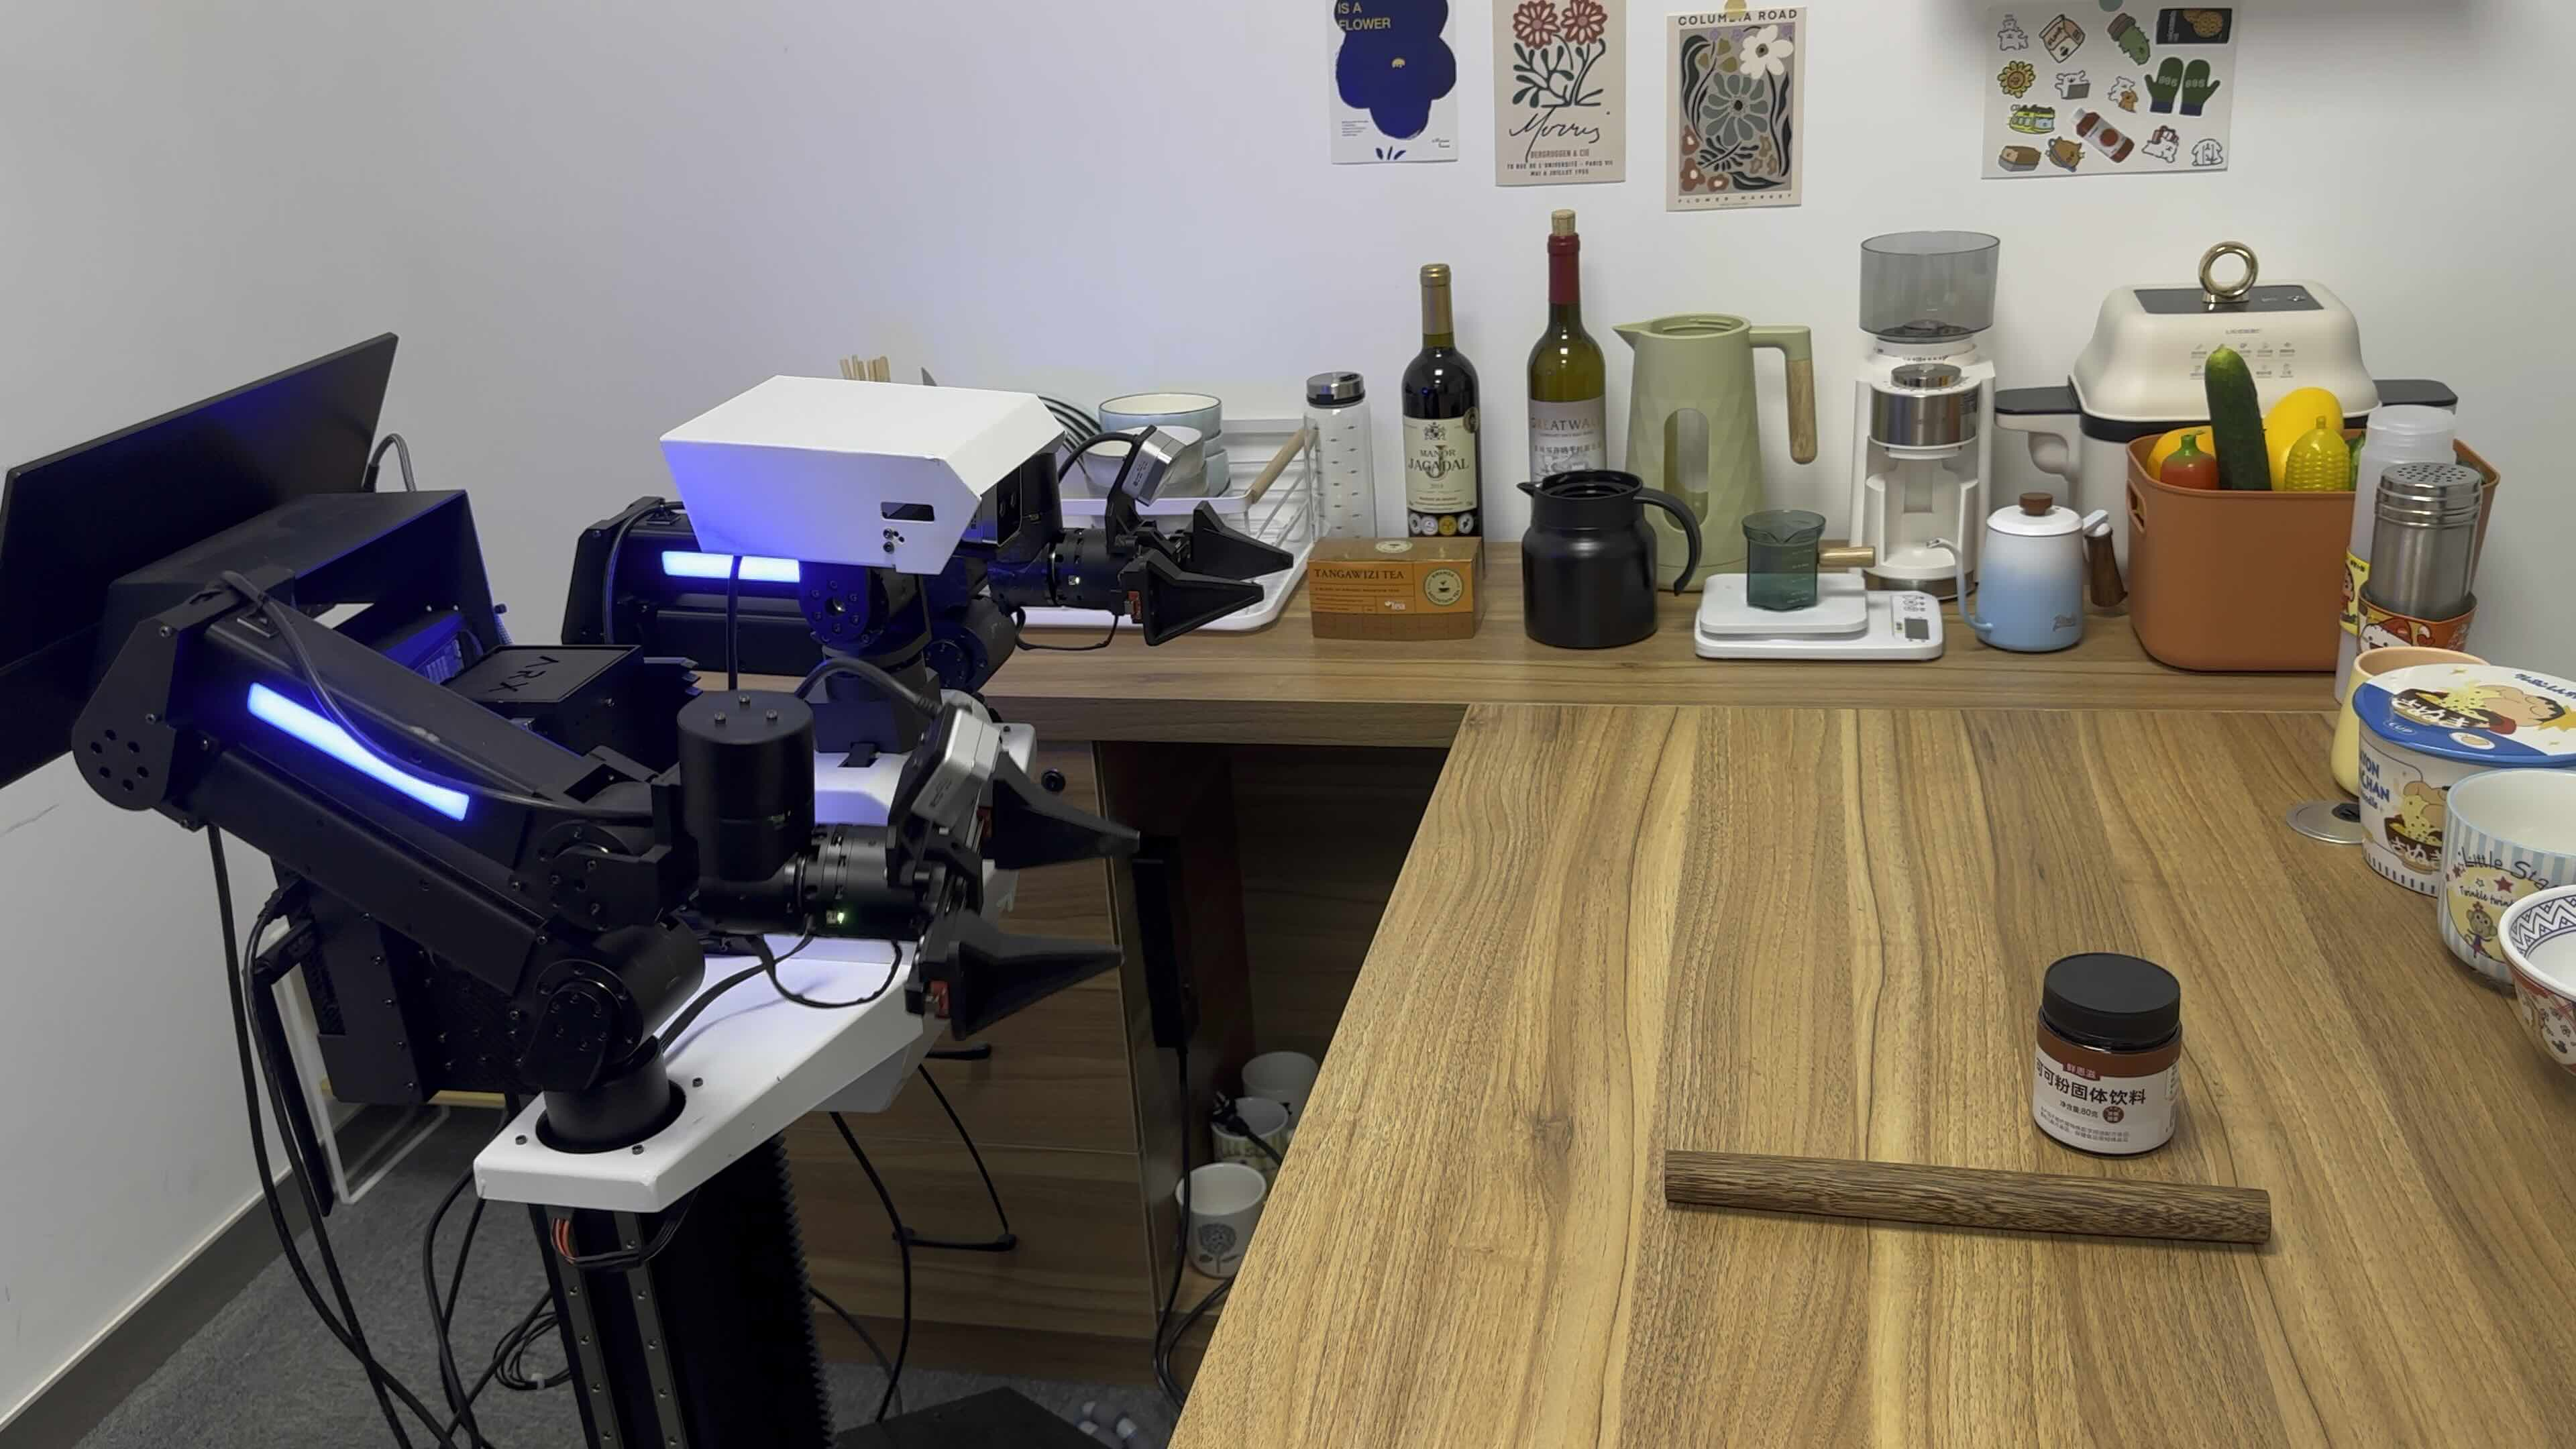}}
        & % Column separator
        \begin{minipage}[t]{\colCwidth}
            \raggedright
            \textbf{Instruction}: Pick up the cocoa powder bottle that is out of reach.\\
            \textbf{Reasoning}:\\
            \textsf{Scene description}: The cocoa power bottle is out of reach. There is a wooden stick nearby. \\
            \textsf{Plan}:  1. Grasp the stick. 2. Sweep the cocoa powder bottle closer with the stick and put down the stick. 3. Pick up the cocoa powder bottle.
        \end{minipage} \\ % End of table row

        \bottomrule % Bottom rule line
    \end{tabular}
    \vspace{2pt}
    \caption{\textbf{Reasoning examples for generalizable planning.}}
    \label{tab:generalizable_plan_reasoning_eg}
\end{table}
