# Supplementary material for: ReFineVLA: Multimodal Reasoning-Aware Generalist Robotic Policies via Teacher-Guided Fine-Tuning
Source: arXiv:2604.17800 source file (2026-04-20)
Supplement: Supplementary file 3 [file table.tex]

% Set the column widths as fractions of \linewidth
% Adjust these fractions as needed.
% Ensure the sum of fractions is slightly less than 1.0 to leave space for \tabcolsep.
\setlength{\colAwidth}{0.25\linewidth}
\setlength{\colBwidth}{0.1\linewidth}
\setlength{\colCwidth}{0.7\linewidth}
\setlength{\figurewidth}{\colAwidth}

\begin{table}[H] % Use htbp for more placement options
    \centering
    \small % Use smaller font size

    % Define the table structure:
    % Column 1: aligned center for images using \adjustbox
    % Column 2: aligned left, controlled by \minipage for captions
    \begin{tabular}{ll}
        \toprule % Top rule line

        % --- First Row: Hotpot ---
        % Image: Use adjustbox to align the top
        \adjustbox{valign=\imagevalign}{\includegraphics[width=\figurewidth]{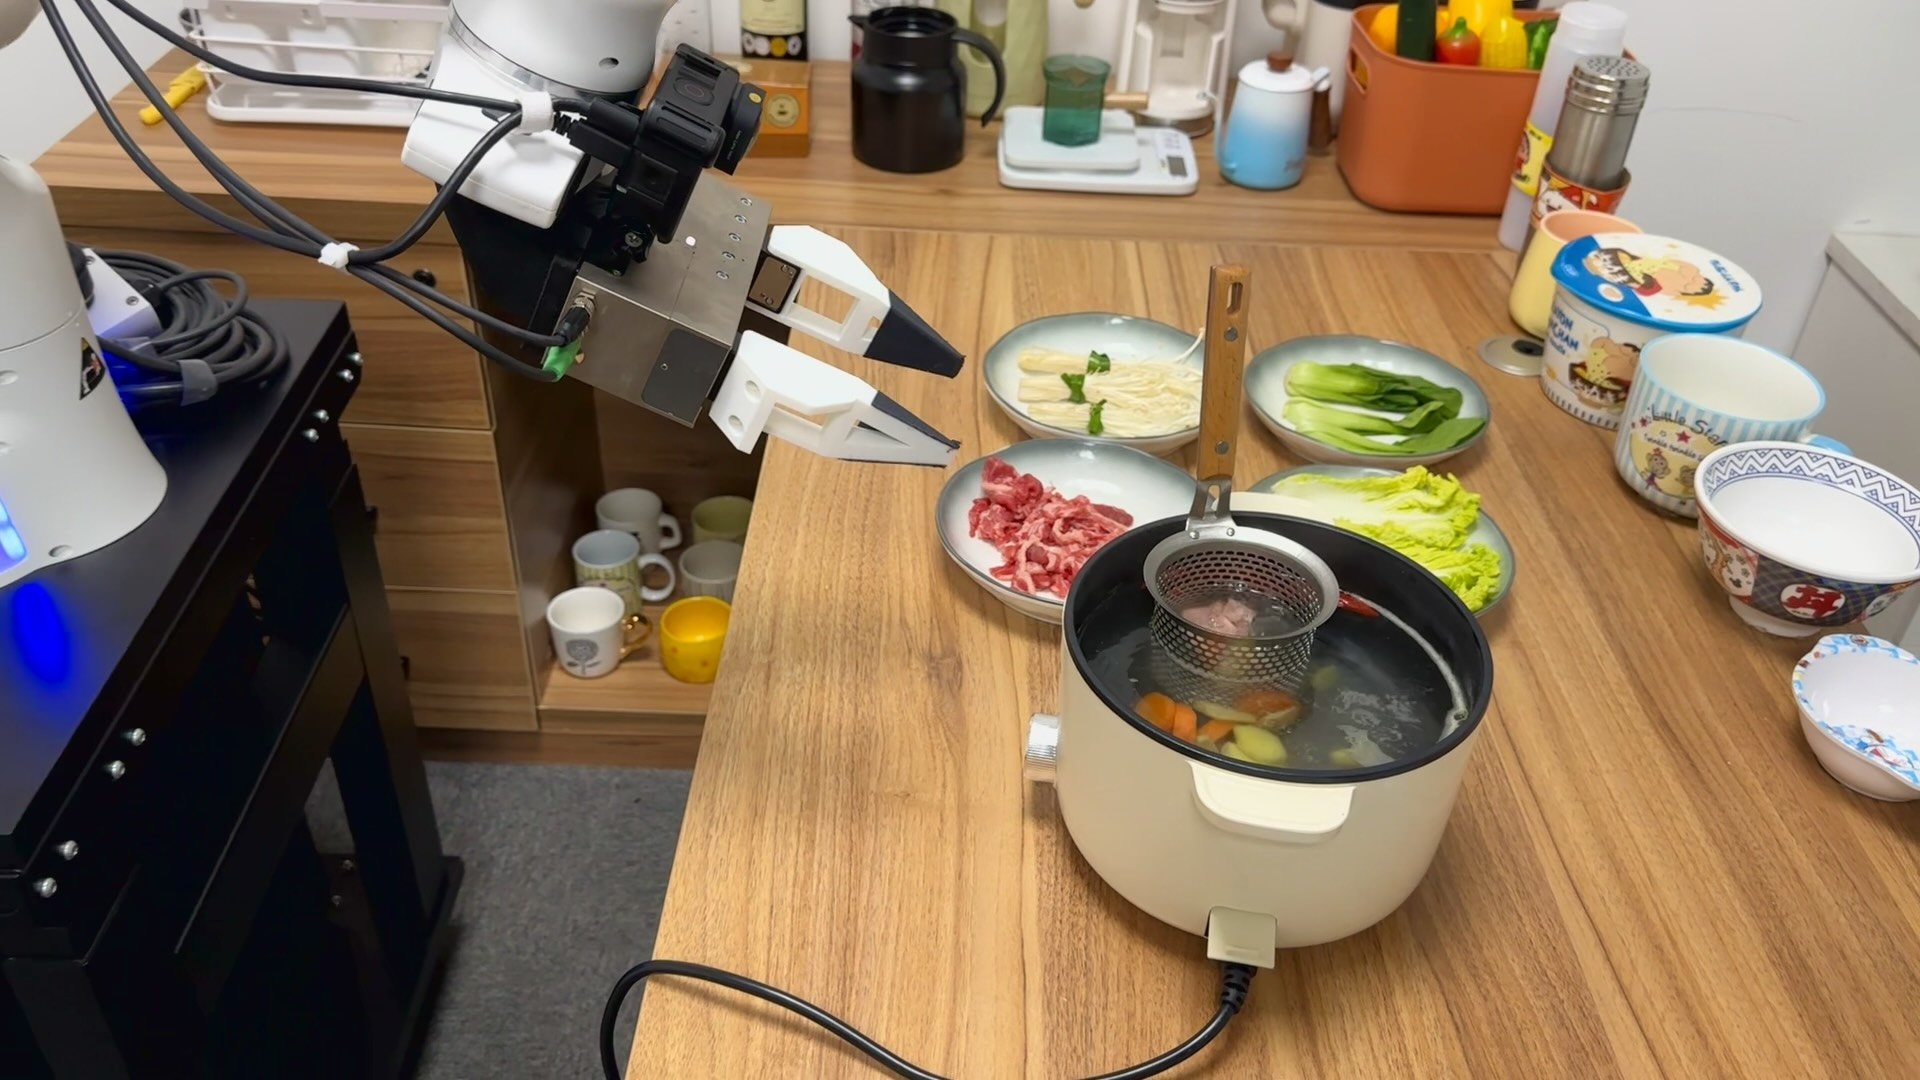}}
        & % Column separator
        % Caption: Place all text in a minipage, use [\imagevalign] for top alignment
        \begin{minipage}[\imagevalign]{\colCwidth}
            \raggedright % Recommended in narrow columns to avoid excessive spacing
            \textbf{Instruction}: Dip the beef for me. \\
            \textbf{Human}: \textit{Could you also dip another vegetable for me?} \\
            \textbf{Robot}: \textit{Sure! Would you like green bok choy, enoki mushrooms, or cabbage?} \\
            \textbf{Human}: \textit{I want some green bok choy.} \\
            \textbf{Reasoning}:\\
            \textsf{Scene description}: Some of the beef is in the hotpot strainer.  \textit{The green bok choy is on the top-left plate.} \\
            \textsf{Plan}: 1. Put the beef into the hotpot strainer. \textit{2. Put the green bok choy into the hotpot strainer.} 3. Wait for the ingredients to cook and then pick up the hotpot strainer. \\
            \textsf{What I have done}: 1. Put the beef into the hotpot strainer. \\
            \textsf{Now I need to}: \textit{Put the green bok choy into the hotpot strainer.}
        \end{minipage} \\ % End of table row
        \midrule % Mid rule line

        % --- Second Row: Tomato ---
        \adjustbox{valign=\imagevalign}{\includegraphics[width=\figurewidth]{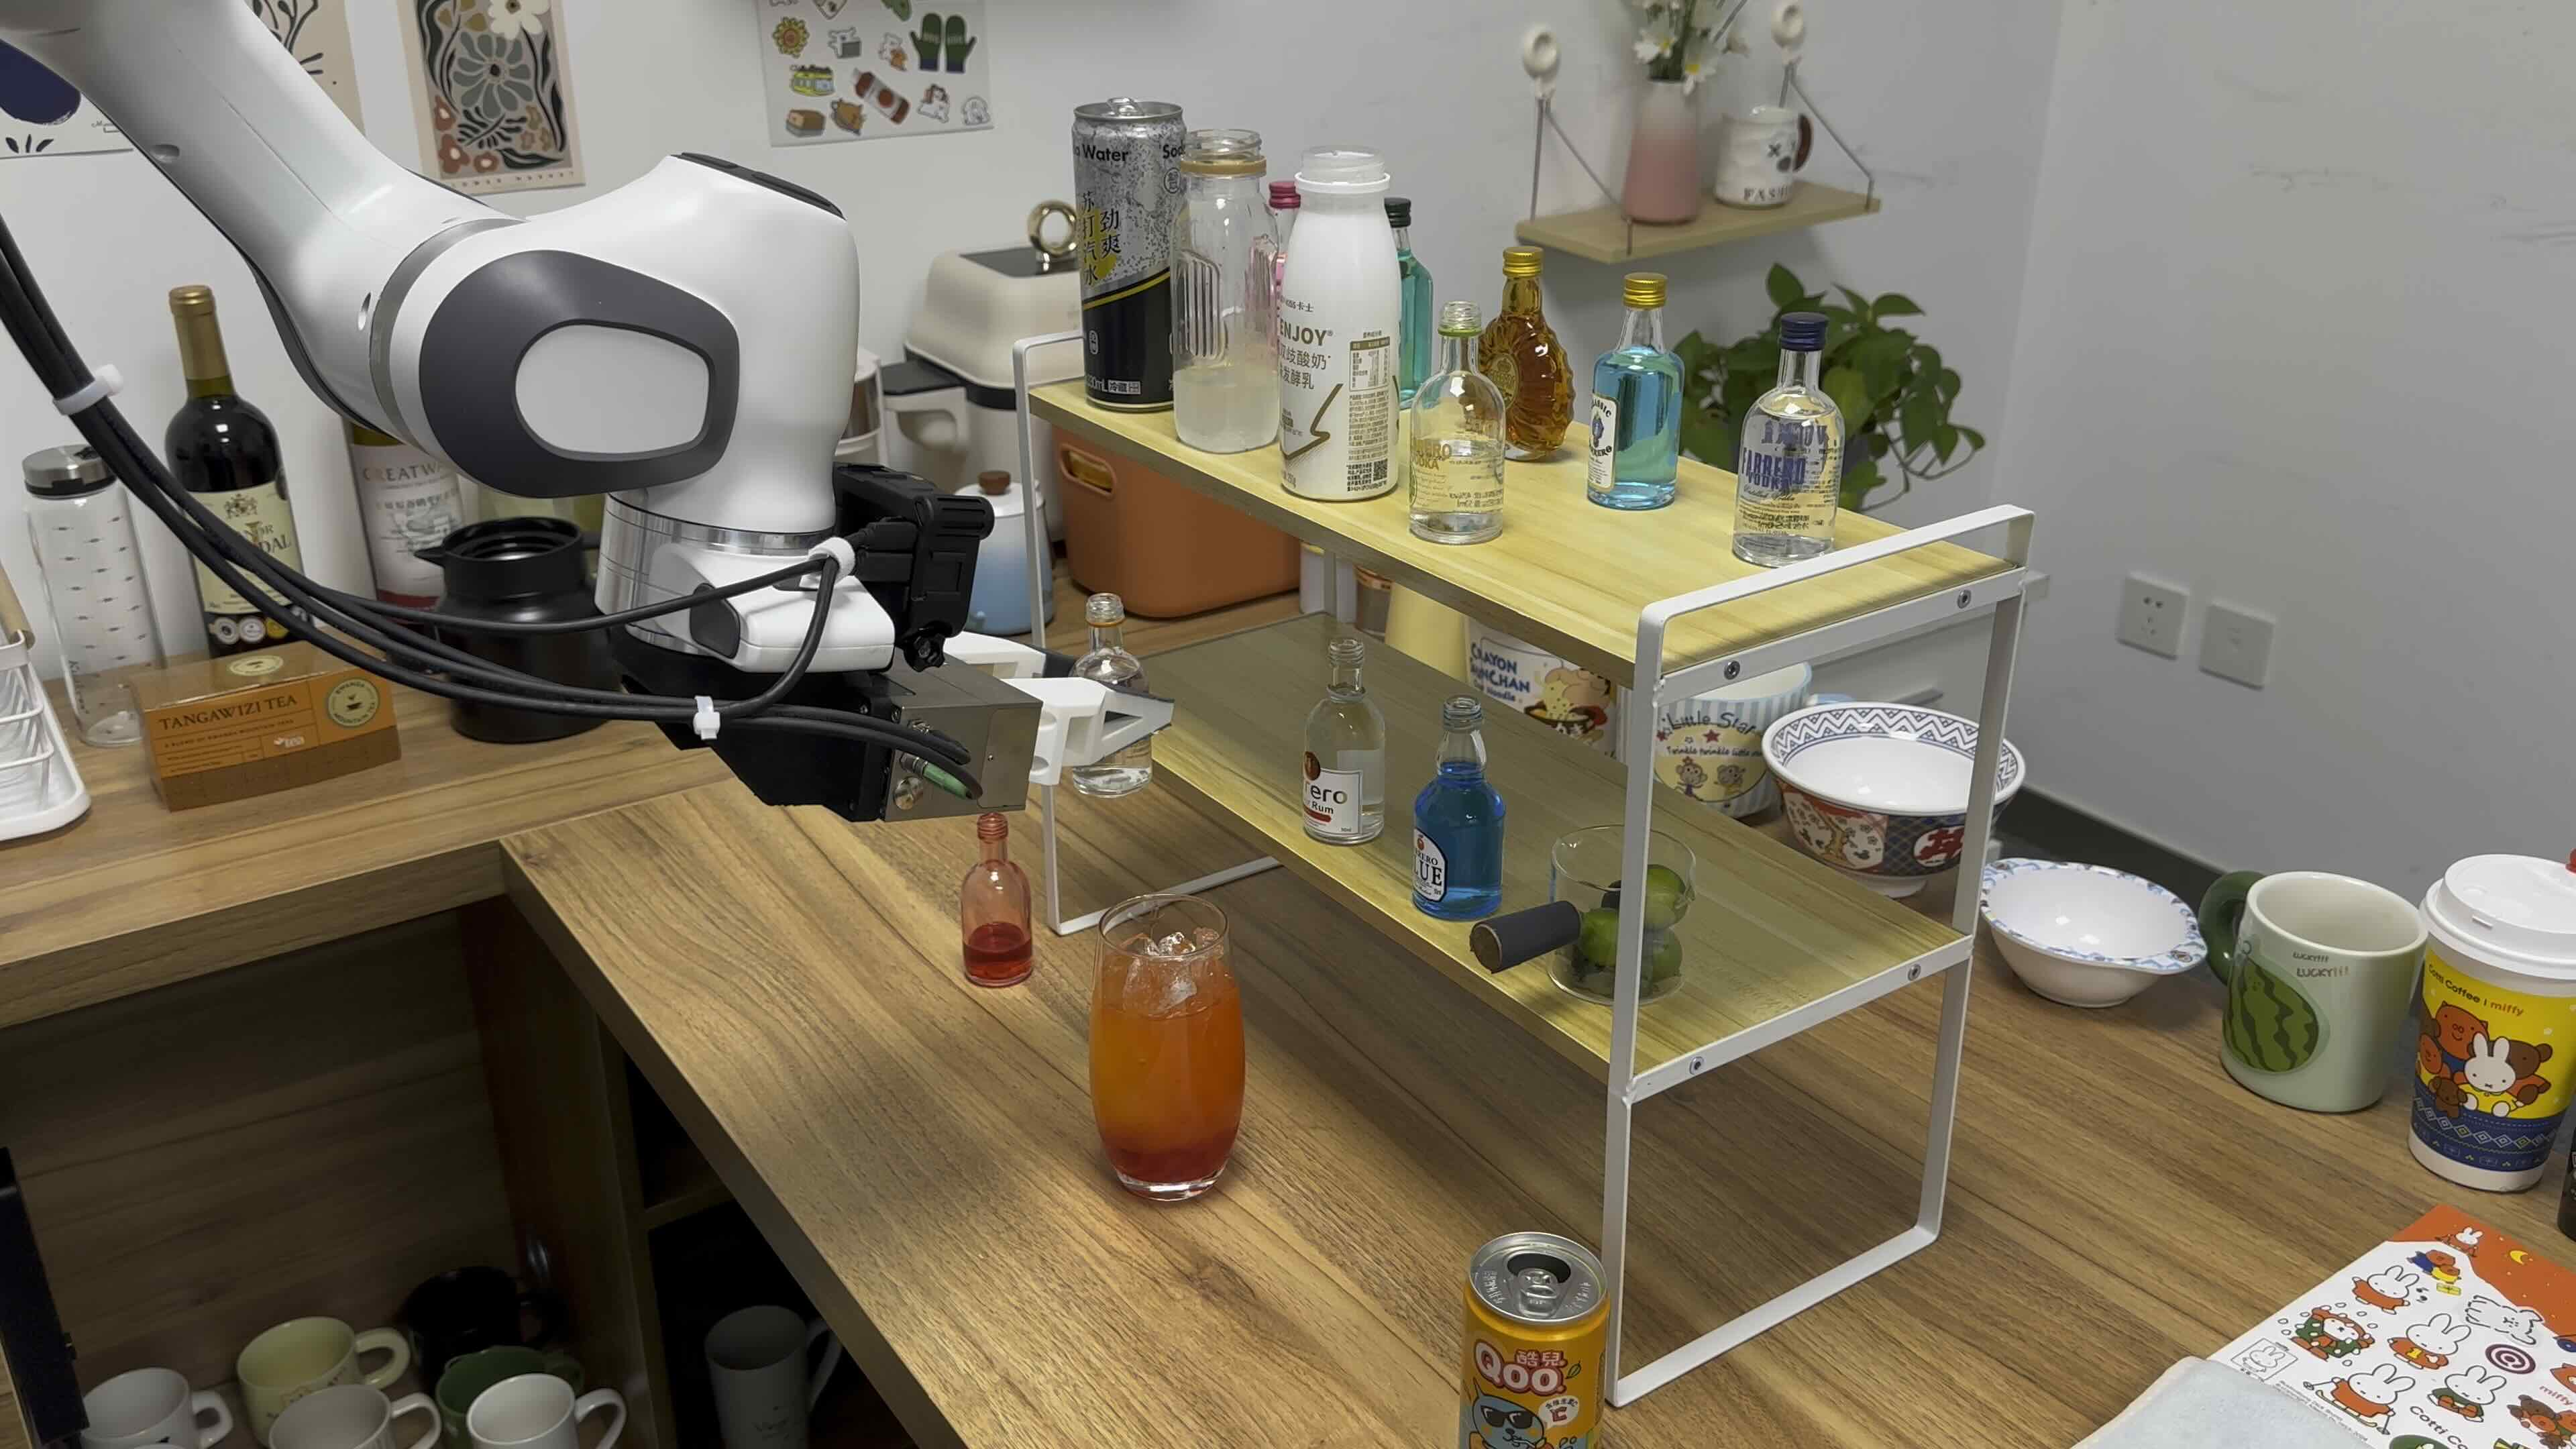}}
        & % Column separator
        \begin{minipage}[\imagevalign]{\colCwidth}
            \raggedright
            \textbf{Instruction}: Make me a cup of \texttt{Vodka Sunrise}. \\
            \textbf{Human}: \textit{I don't want orange vodka, I want lemon-flavored one.} \\
            \textbf{Reasoning}:\\
            \textsf{Scene description}: The grenadine syrup and orange juice have been poured into the glass. \textit{The lemon-flavored vodka is the second from the right on the top shelf.} \\
            \textsf{Plan}:  1. Pour the grenadine syrup into the glass. 2. Pour the orange juice into the glass. \textit{3. Put down the orange vodka, and retrieve the lemon vodka.} \\
            \textsf{What I have done}: 1. Pour the grenadine syrup into the glass. 2. Pour the orange juice into the glass. \\
            \textsf{Now I need to}: \textit{Put down the orange vodka, and retrieve the lemon vodka.}
        \end{minipage} \\ % End of table row

        \bottomrule % Bottom rule line
    \end{tabular}
    \vspace{2pt}
    \caption{\textbf{Reasoning examples for natural human robot interaction.}}
    \label{tab:interaction_reasoning_eg}
\end{table}
