# Supplementary material for: ReFineVLA: Multimodal Reasoning-Aware Generalist Robotic Policies via Teacher-Guided Fine-Tuning
Source: arXiv:2604.17800 source file (2026-04-20)
Supplement: Supplementary file 4 [file table.tex]

% Set the column widths as fractions of \linewidth
% Adjust these fractions as needed.
% Ensure the sum of fractions is slightly less than 1.0 to leave space for \tabcolsep.
\setlength{\colAwidth}{0.25\linewidth}
\setlength{\colBwidth}{0.1\linewidth}
\setlength{\colCwidth}{0.7\linewidth}
\setlength{\figurewidth}{\colAwidth}

\begin{table}[H] % Use htbp for more placement options
    \centering
    \small % Use smaller font size

    % Define the table structure:
    % Column 1: aligned center for images using \adjustbox
    % Column 2: aligned left, controlled by \minipage for captions
    \begin{tabular}{ll}
        \toprule % Top rule line

        % --- First Row: Direct Sprite ---
        % Image: Use adjustbox to align the top
        \adjustbox{valign=t}{\includegraphics[width=\figurewidth]{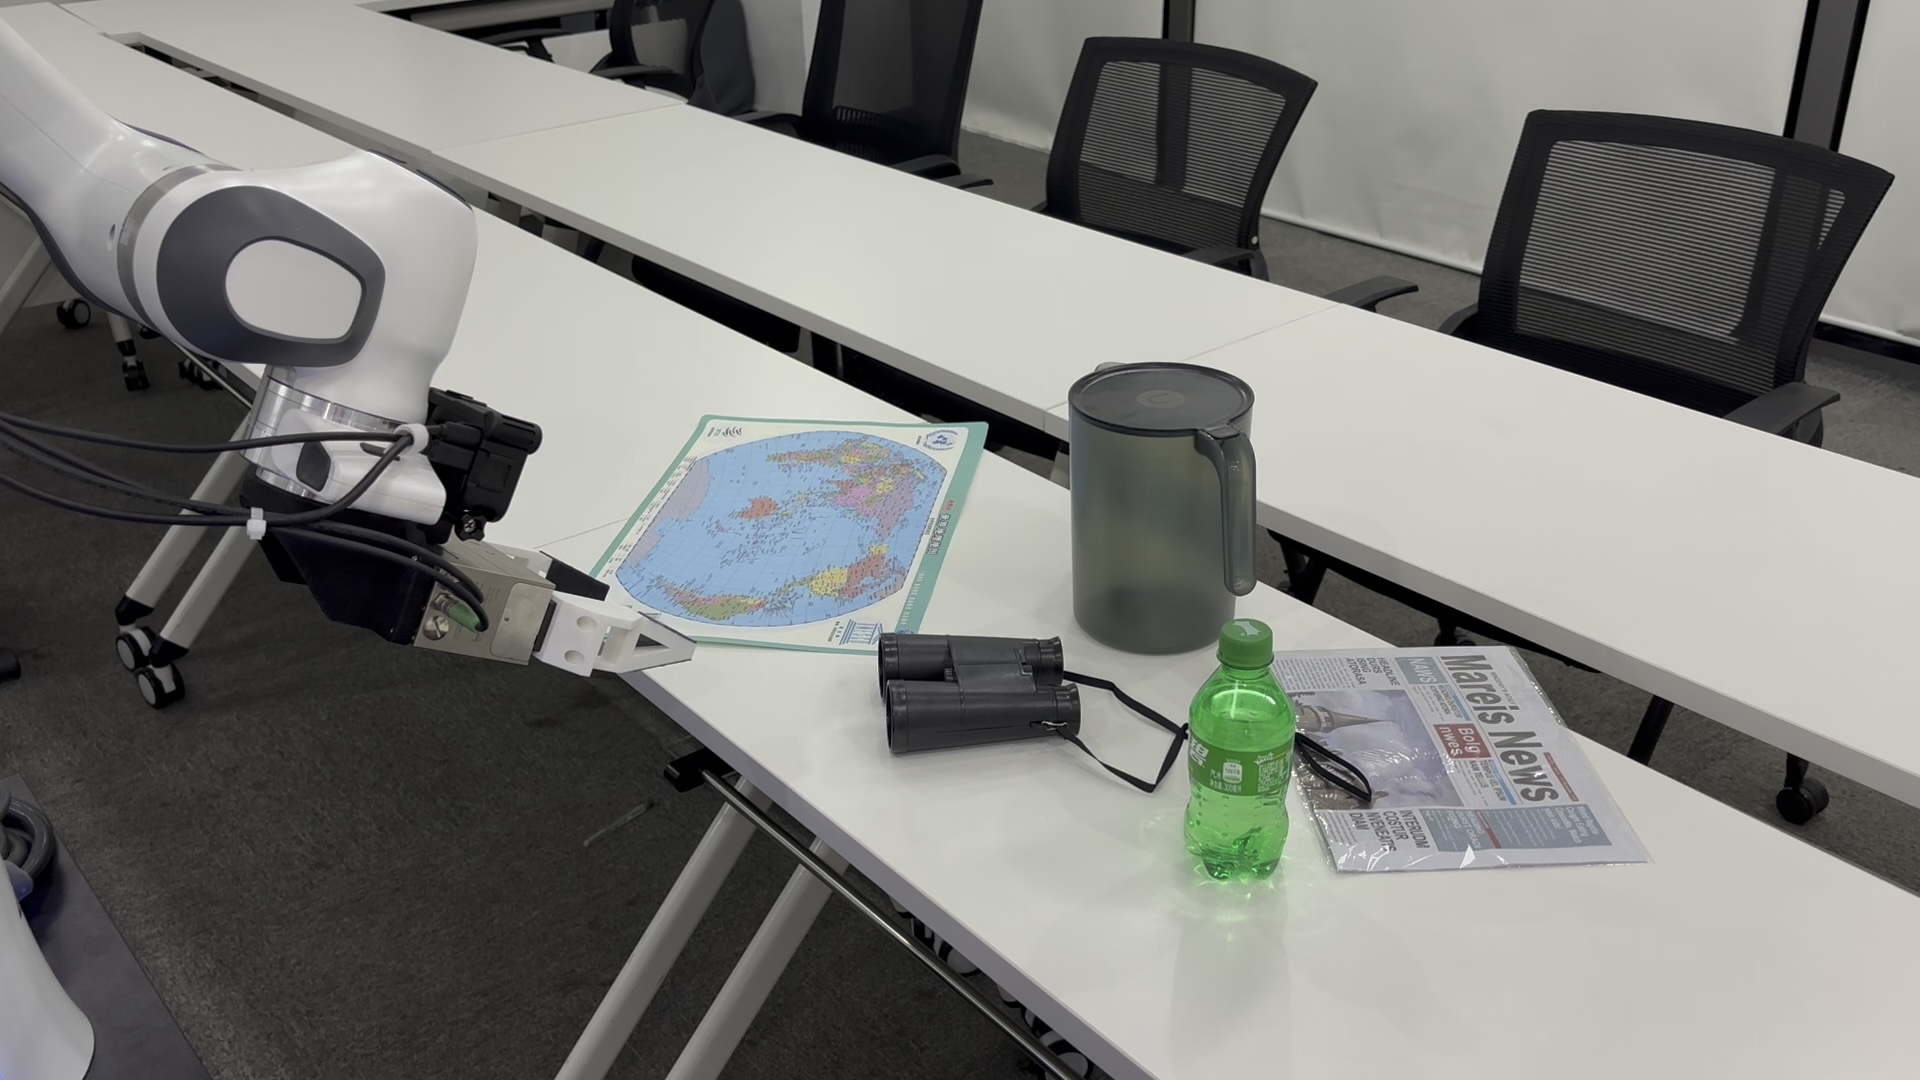}}
        & % Column separator
        % Caption: Place all text in a minipage, use [t] for top alignment
        \begin{minipage}[t]{\colCwidth}
            \raggedright % Recommended in narrow columns to avoid excessive spacing
            \textbf{Instruction}: Bring me the Sprite. \\
            \textbf{Reasoning}:\\
            I need to pick up green Sprite, which is a model of a drink, located on the right side of the table. \\
        \end{minipage} \\ % End of table row
        \midrule % Mid rule line

        % --- Second Row: Spatial lantern ---
        \adjustbox{valign=t}{\includegraphics[width=\figurewidth]{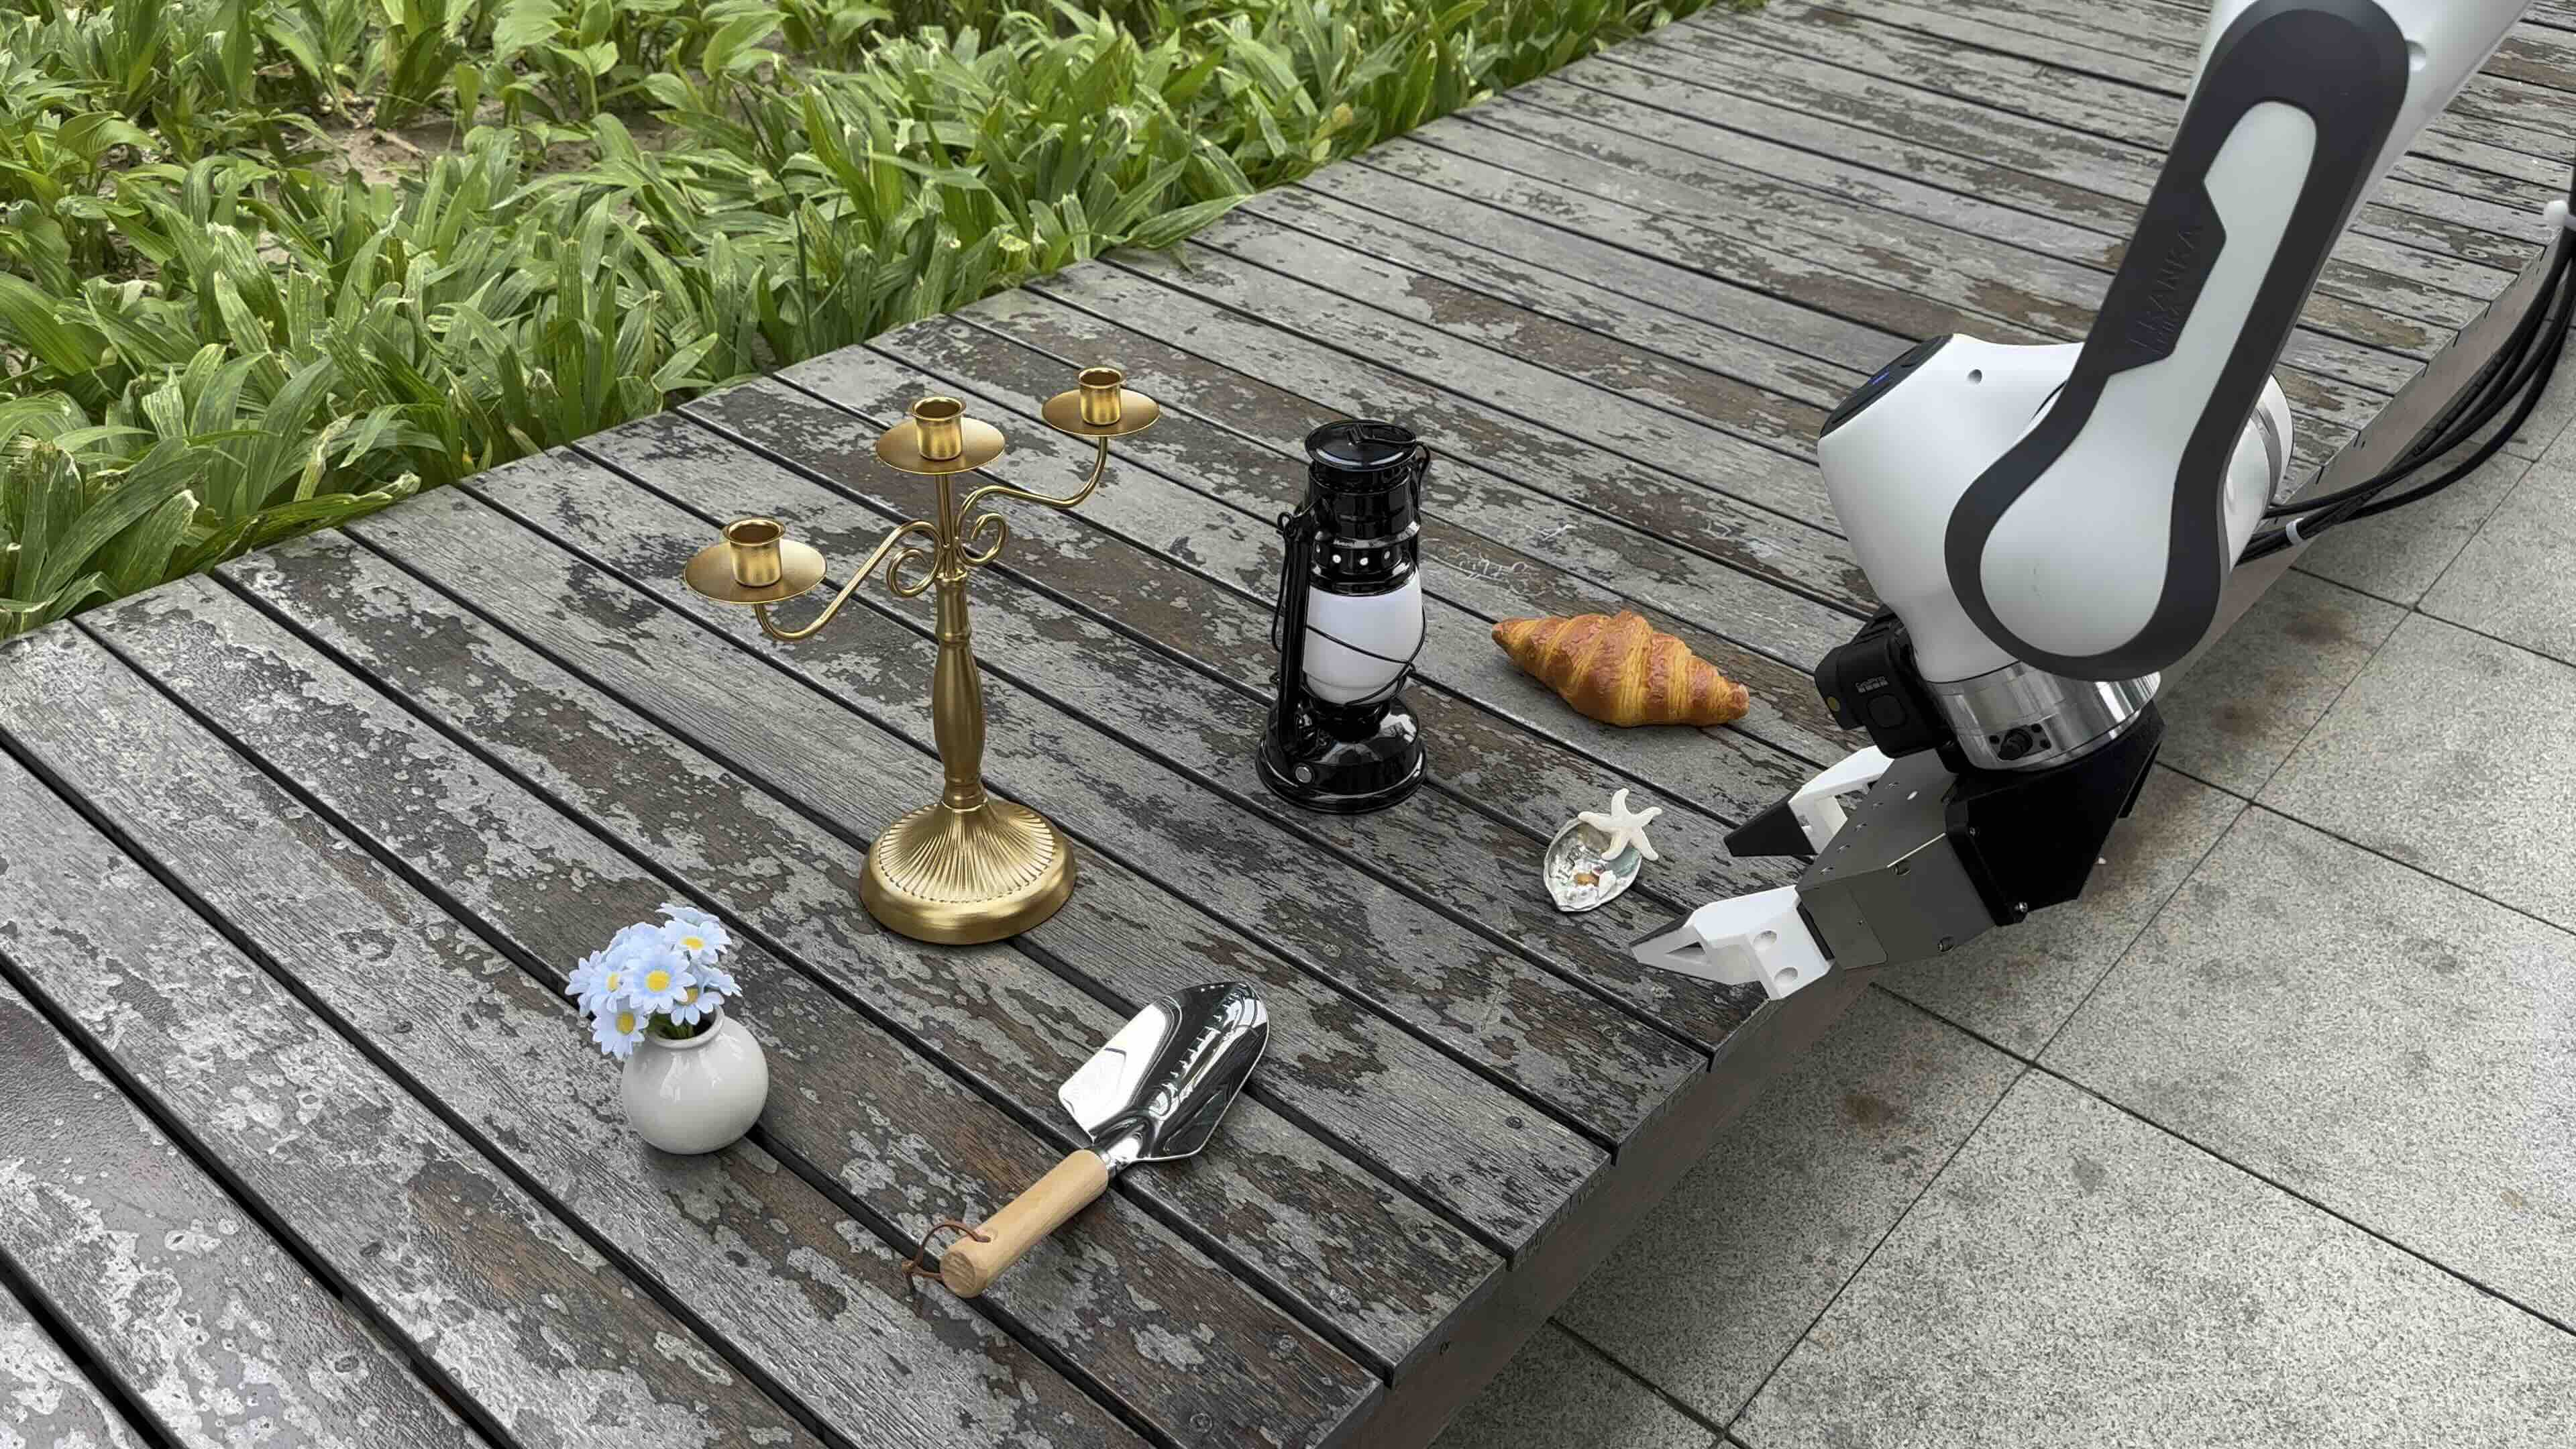}}
        & % Column separator
        \begin{minipage}[t]{\colCwidth}
            \raggedright
            \textbf{Instruction}: Give me the object behind the seashell.\\
            \textbf{Reasoning}: \\
            I need to pick up the lantern to the left of the croissant, which is black with a metal structure, and holds light and can be carried.
        \end{minipage} \\ % End of table row
        \midrule % Mid rule line

        % --- Third Row: Attribute Clock ---
        \adjustbox{valign=t}{\includegraphics[width=\figurewidth]{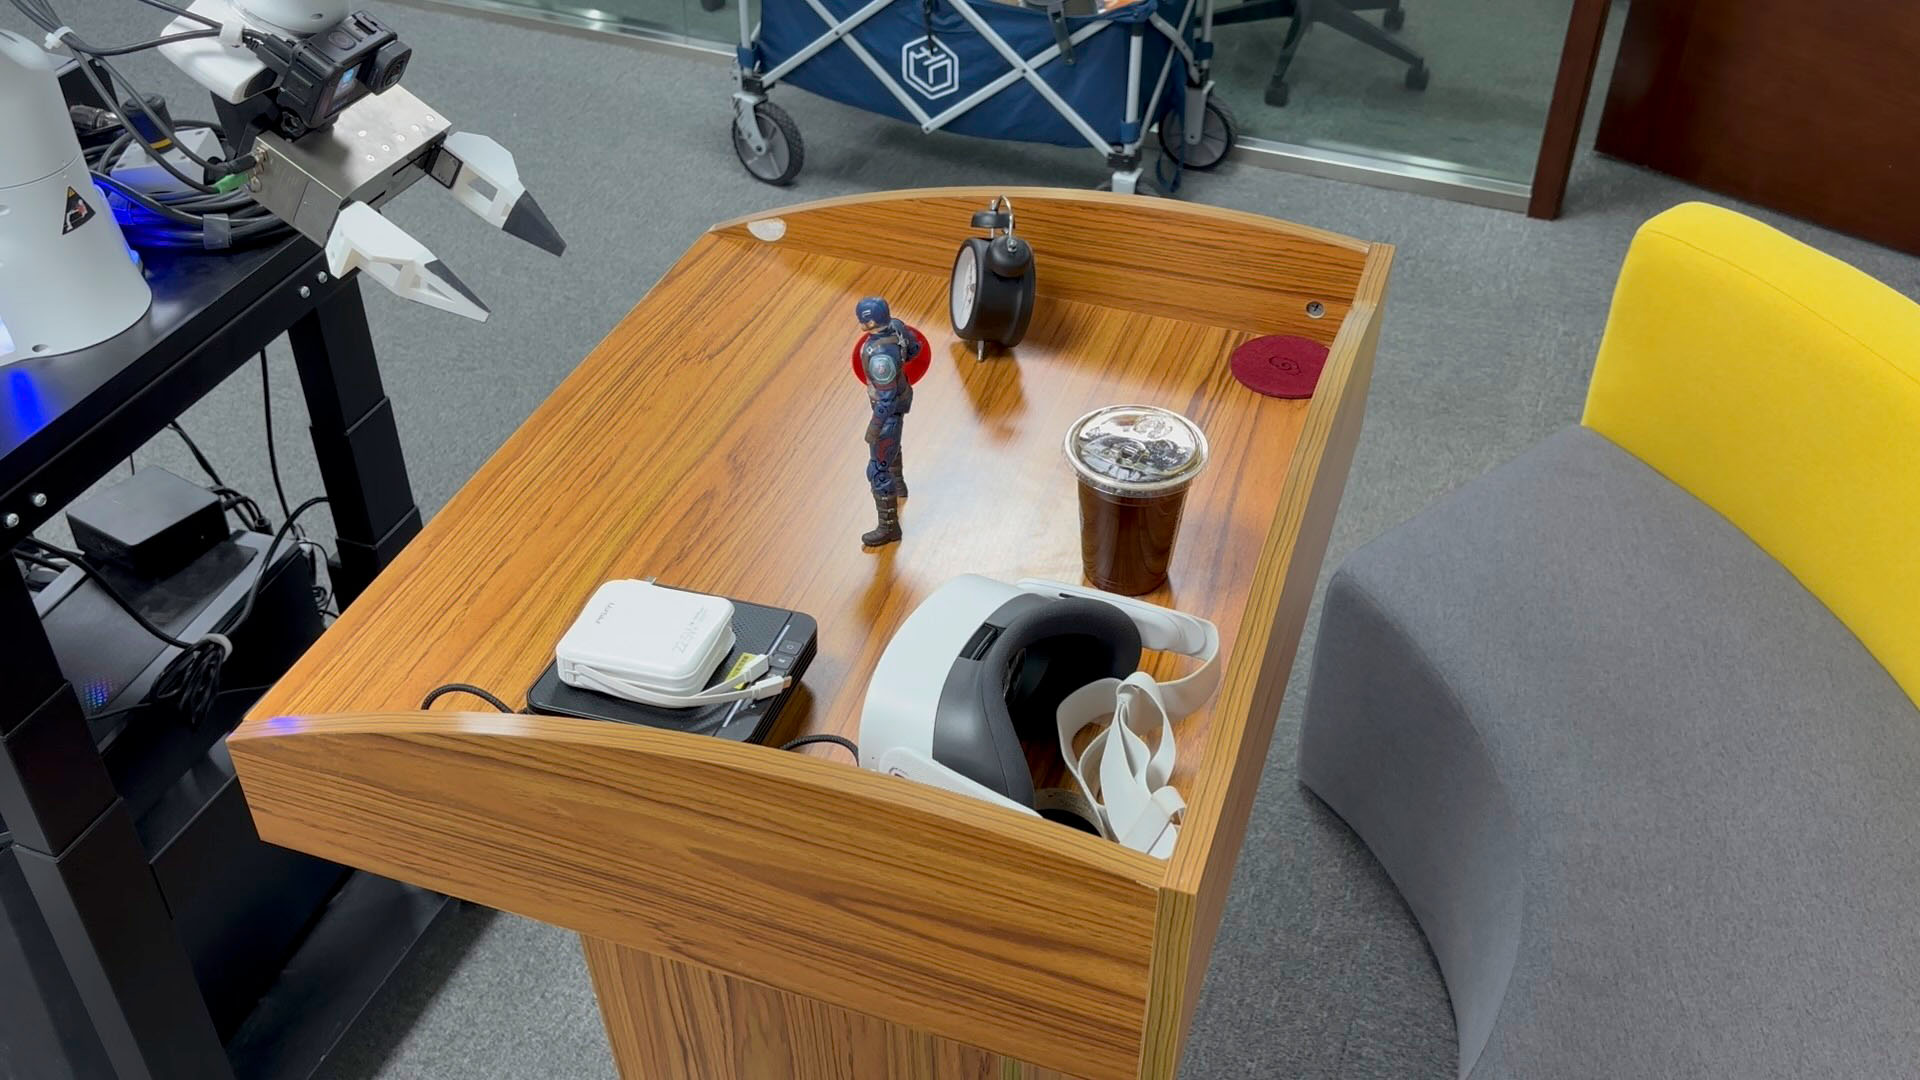}}
        & % Column separator
        \begin{minipage}[t]{\colCwidth}
            \raggedright
            \textbf{Instruction}: Hand me the object which is black and round. \\
            \textbf{Reasoning}: \\
            I need to pick up the alarm clock sitting on the left side of the table. \\
        \end{minipage} \\ % End of table row
        \midrule % Mid rule line

        % --- Fourth Row: Semantic Magnifier ---
        \adjustbox{valign=t}{\includegraphics[width=\figurewidth]{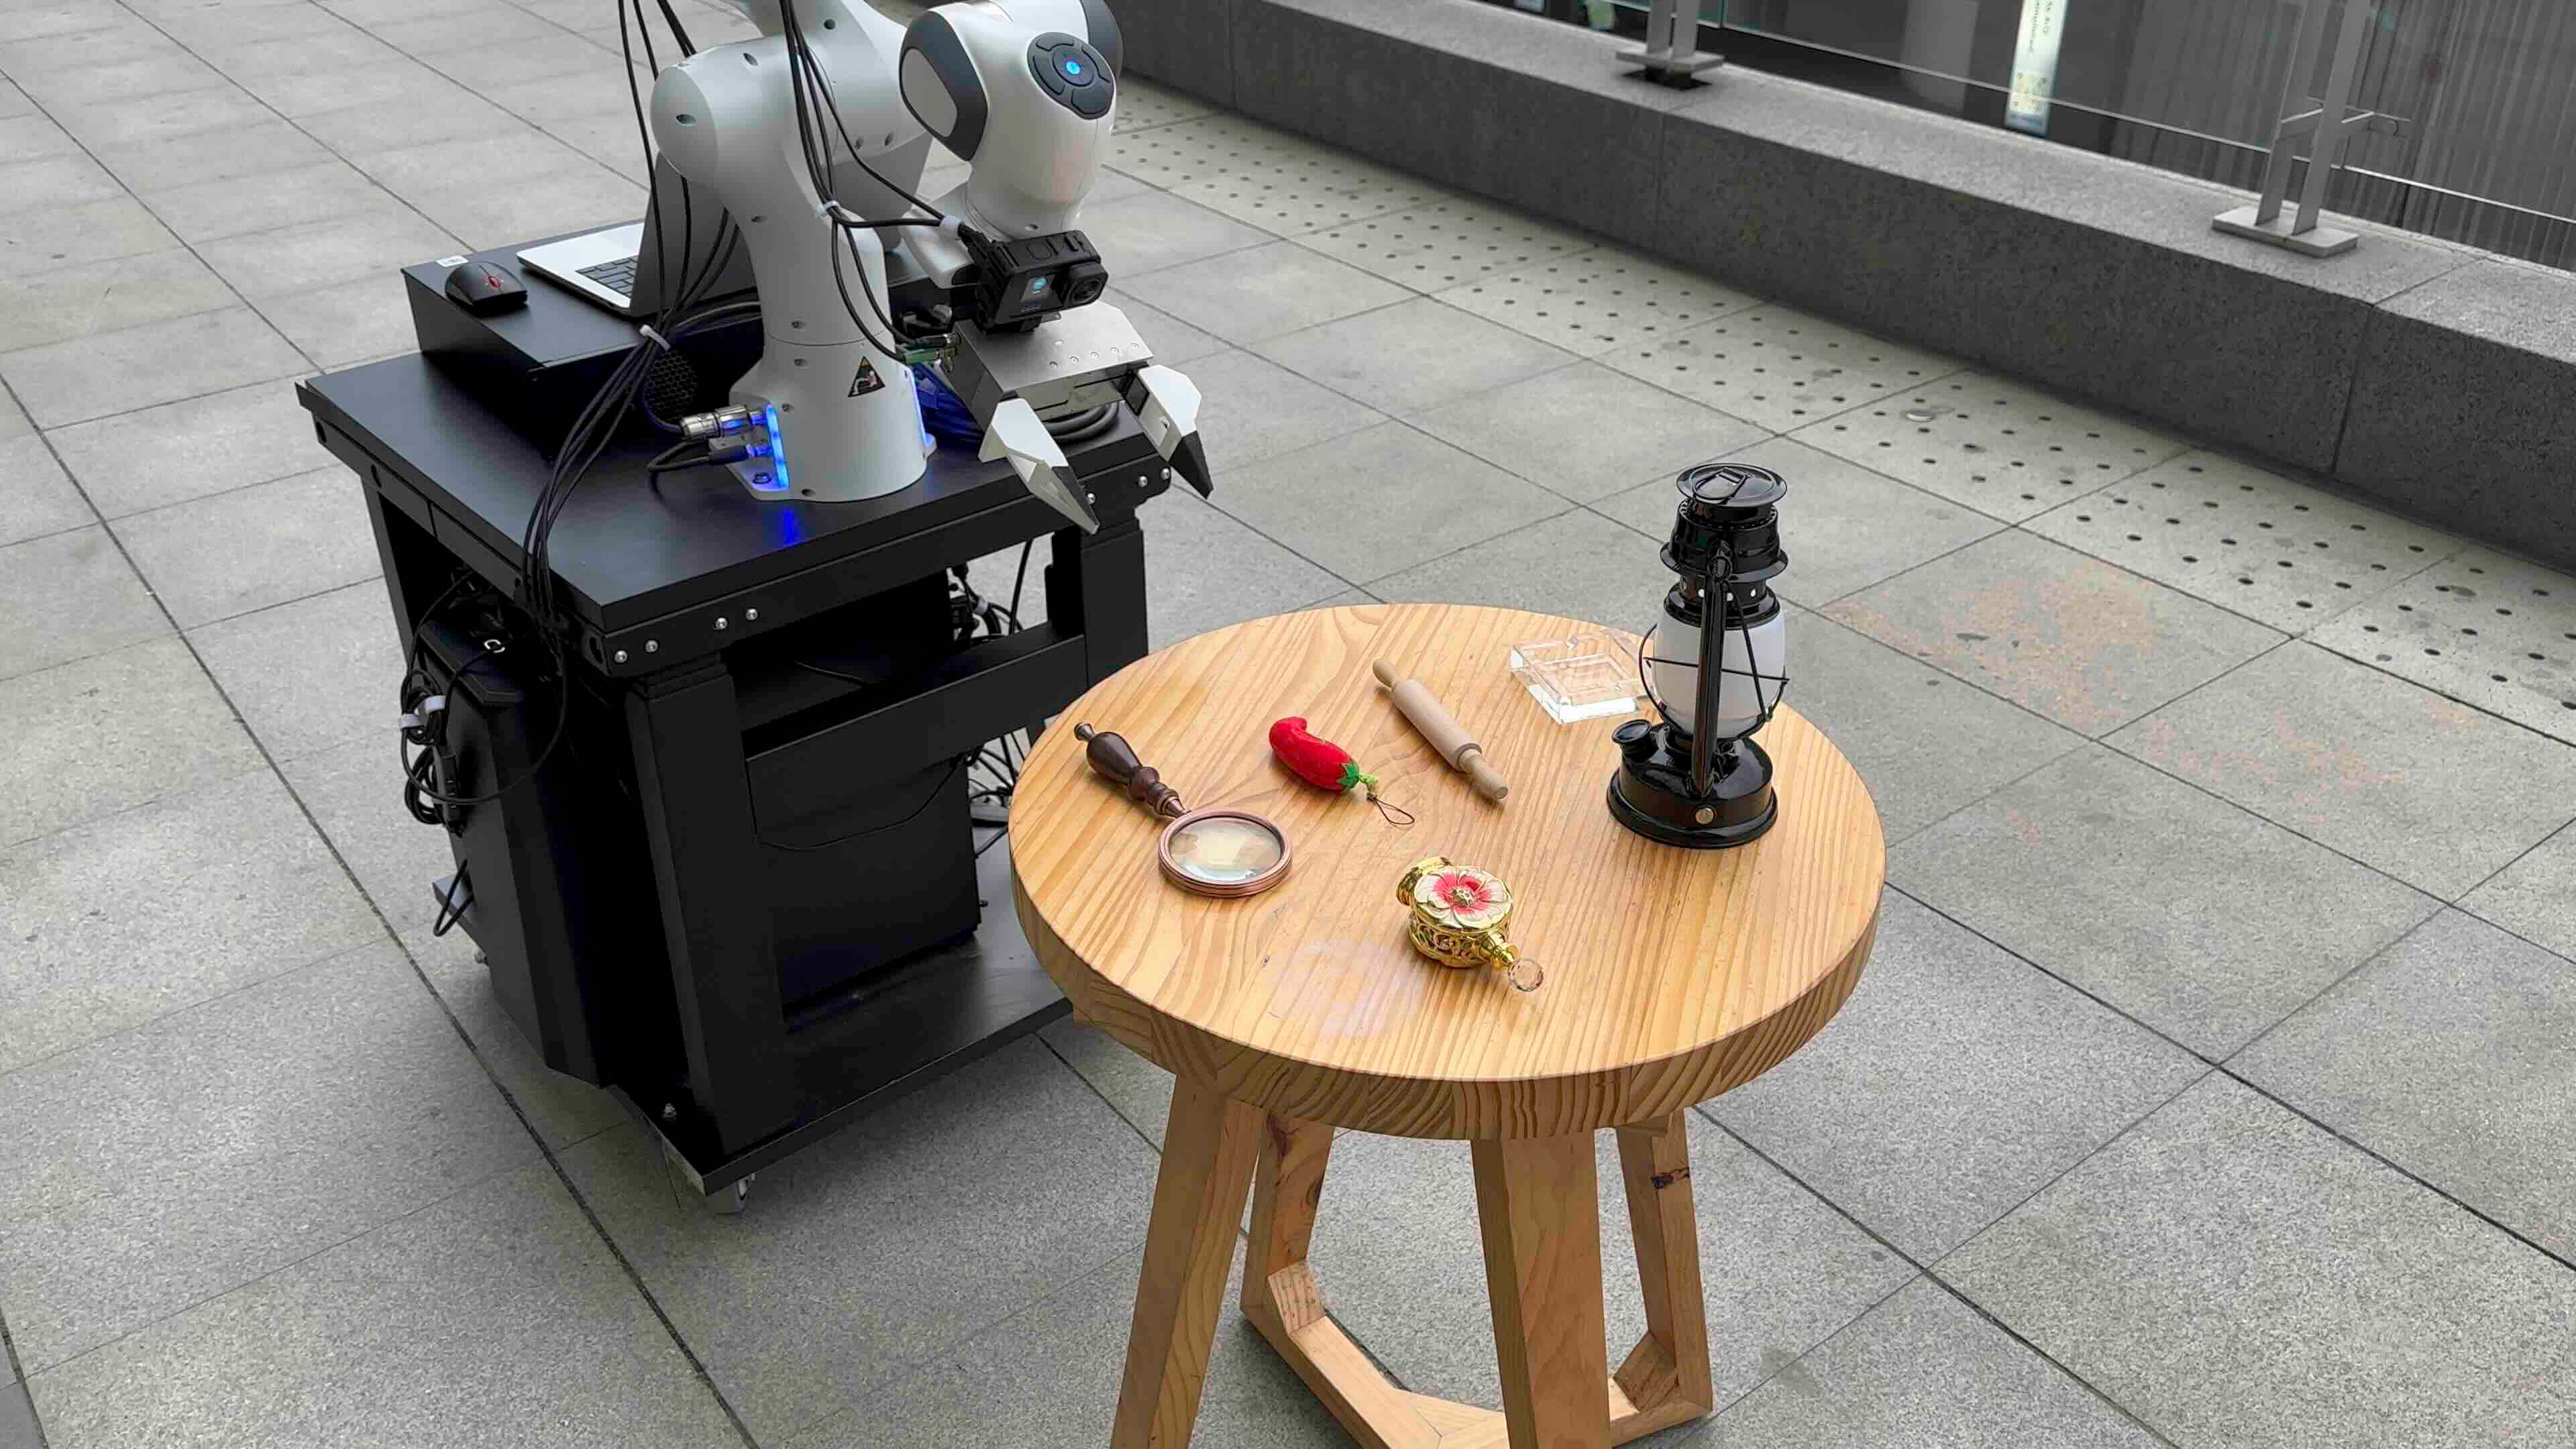}}
        & % Column separator
        \begin{minipage}[t]{\colCwidth}
            \raggedright
            \textbf{Instruction}: I need something to get a closer look at this fine print. \\
            \textbf{Reasoning}: \\
            I need to pick up the magnifying glass, which is to the right of the red pepper, and has a wooden handle and a circular lens. \\
        \end{minipage} \\ % End of table row

        \bottomrule % Bottom rule line
    \end{tabular}
    \vspace{2pt}
    \caption{\textbf{Reasoning examples for \texttt{Open-World} visual grounding.}}
    \label{tab:open_world_visual_grounding_reasoning_eg}
\end{table}
