# Supplementary material for: ReFineVLA: Multimodal Reasoning-Aware Generalist Robotic Policies via Teacher-Guided Fine-Tuning
Source: arXiv:2604.17800 source file (2026-04-20)
Supplement: Supplementary file 5 [file table.tex]

% Set the column widths as fractions of \linewidth
% Adjust these fractions as needed.
% Ensure the sum of fractions is slightly less than 1.0 to leave space for \tabcolsep.
\setlength{\colAwidth}{0.25\linewidth}
\setlength{\colBwidth}{0.1\linewidth}
\setlength{\colCwidth}{0.7\linewidth}
\setlength{\figurewidth}{\colAwidth}

\begin{table}[H] % Use htbp for more placement options
    \centering
    \small % Use smaller font size

    % Define the table structure:
    % Column 1: aligned center for images using \adjustbox
    % Column 2: aligned left, controlled by \minipage for captions
    \begin{tabular}{ll}
        \toprule % Top rule line

        % --- First Row: Hotpot ---
        % Image: Use adjustbox to align the top
        \adjustbox{valign=\imagevalign}{\includegraphics[width=\figurewidth]{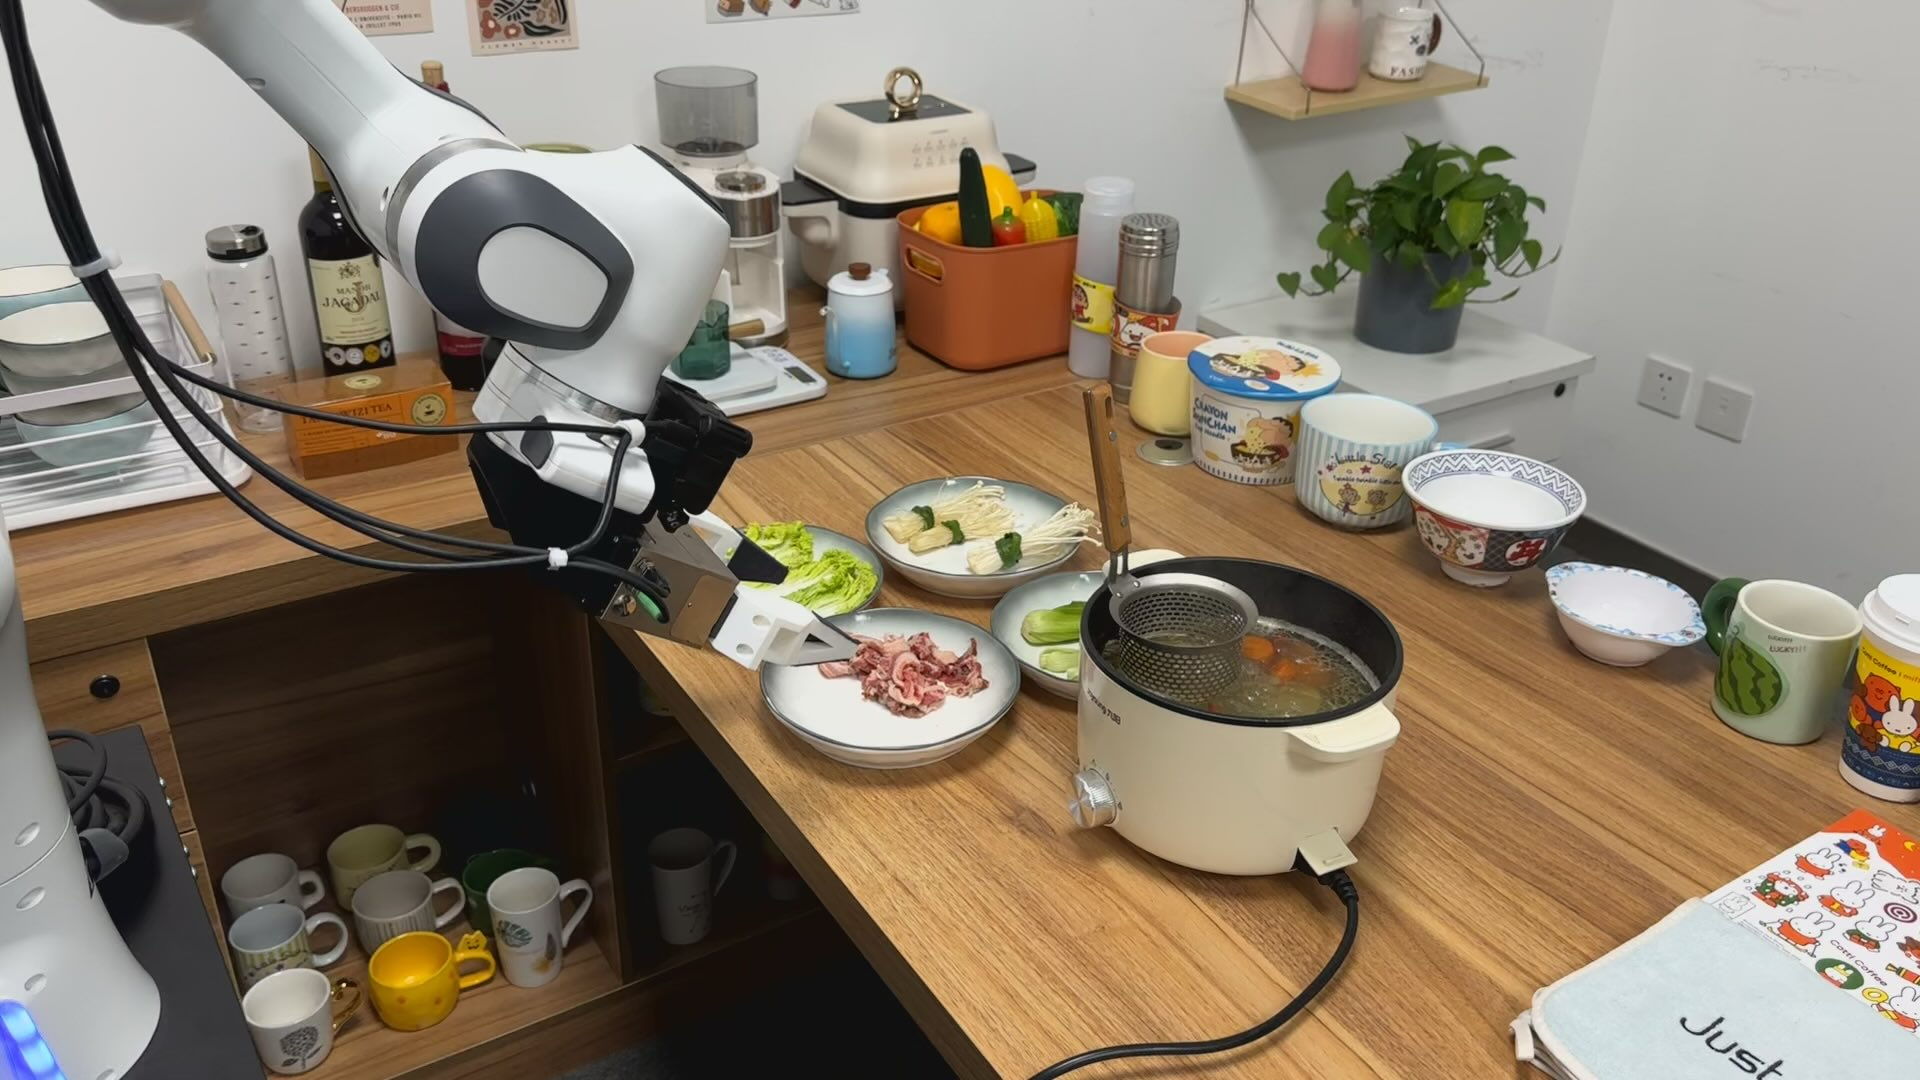}}
        & % Column separator
        \begin{minipage}[\imagevalign]{\colCwidth}
            \raggedright % Recommended in narrow columns to avoid excessive spacing
            \textbf{Instruction}: Dip the beef and the green bok choy. \\
            \textbf{Reasoning}:\\
            \textsf{Scene description}: The beef is located on the bottom-right plate. The green bok choy is on the top-right plate. The pot is in the center-right area of the table and contains a hotpot strainer. \\
            \textsf{Plan}: 1. Put the beef into the hotpot strainer. 2. Put the green bok choy into the hotpot strainer. 3. Wait for the ingredients to cook and then pick up the hotpot strainer. \\
            \textsf{What I have done}: Nothing.\\
            \textsf{Now I need to}: Put the beef into the hotpot strainer.
        \end{minipage} \\ % End of table row
        \midrule % Mid rule line

        % --- Second Row: Tomato ---
        \adjustbox{valign=\imagevalign}{\includegraphics[width=\figurewidth]{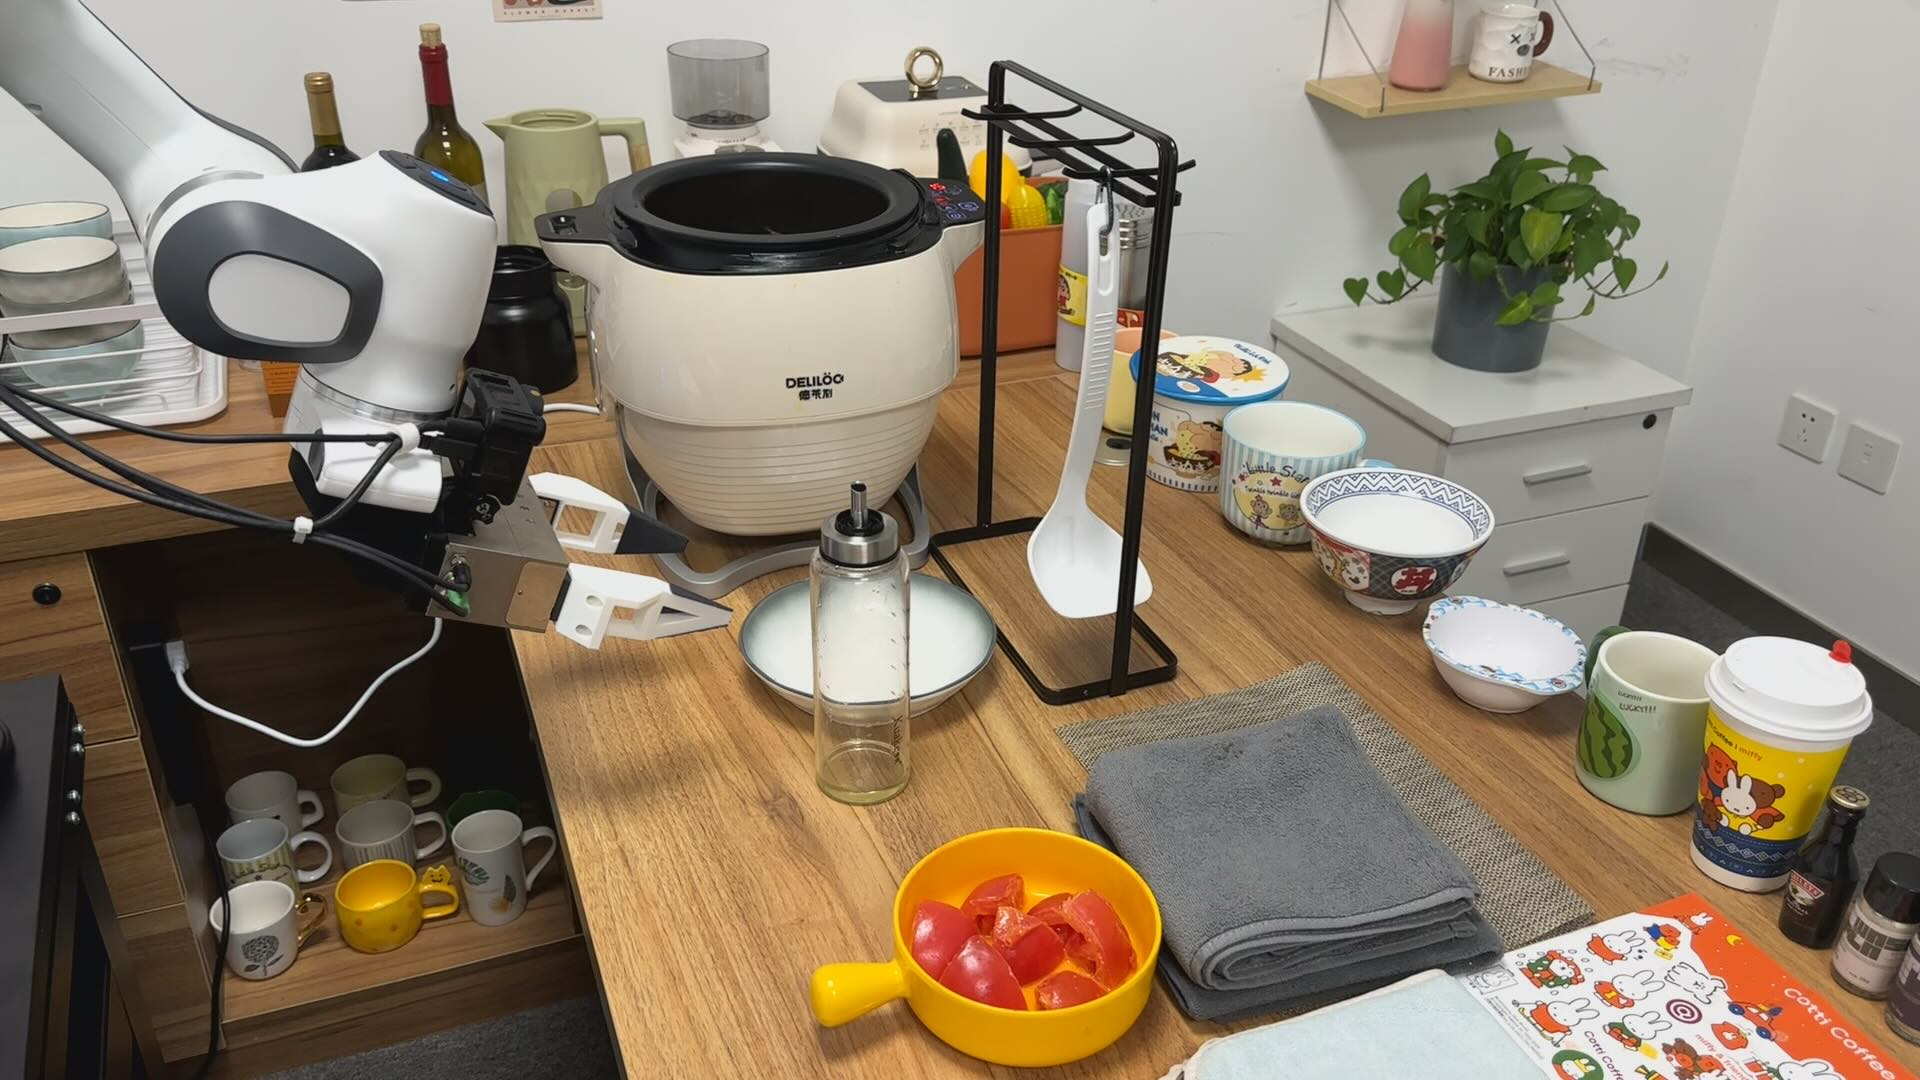}}
        & % Column separator
        \begin{minipage}[\imagevalign]{\colCwidth}
            \raggedright
            \textbf{Instruction}: Make me a plate of tomato-egg scramble. \\
            \textbf{Reasoning}:\\
            \textsf{Scene description}: The oil bottle is located at the front of the table. The cooking machine is on the left side of the table.  \\
            \textsf{Plan}:  1. Pour the oil into the cooking machine. 2. Pour the tomatoes and egg liquid into the cooking machine. 3. Wait for the cooking process to finish, then pick up the spoon. 4. Scoop out the tomato-egg scramble, transfer it onto the plate, and place the spoon into the cooking machine. \\
            \textsf{What I have done}: Nothing.\\
            \textsf{Now I need to}: Pour the oil into the cooking machine.
        \end{minipage} \\ % End of table row
        \midrule % Mid rule line

        % --- Third Row: Fuji ---
        \adjustbox{valign=\imagevalign}{\includegraphics[width=\figurewidth]{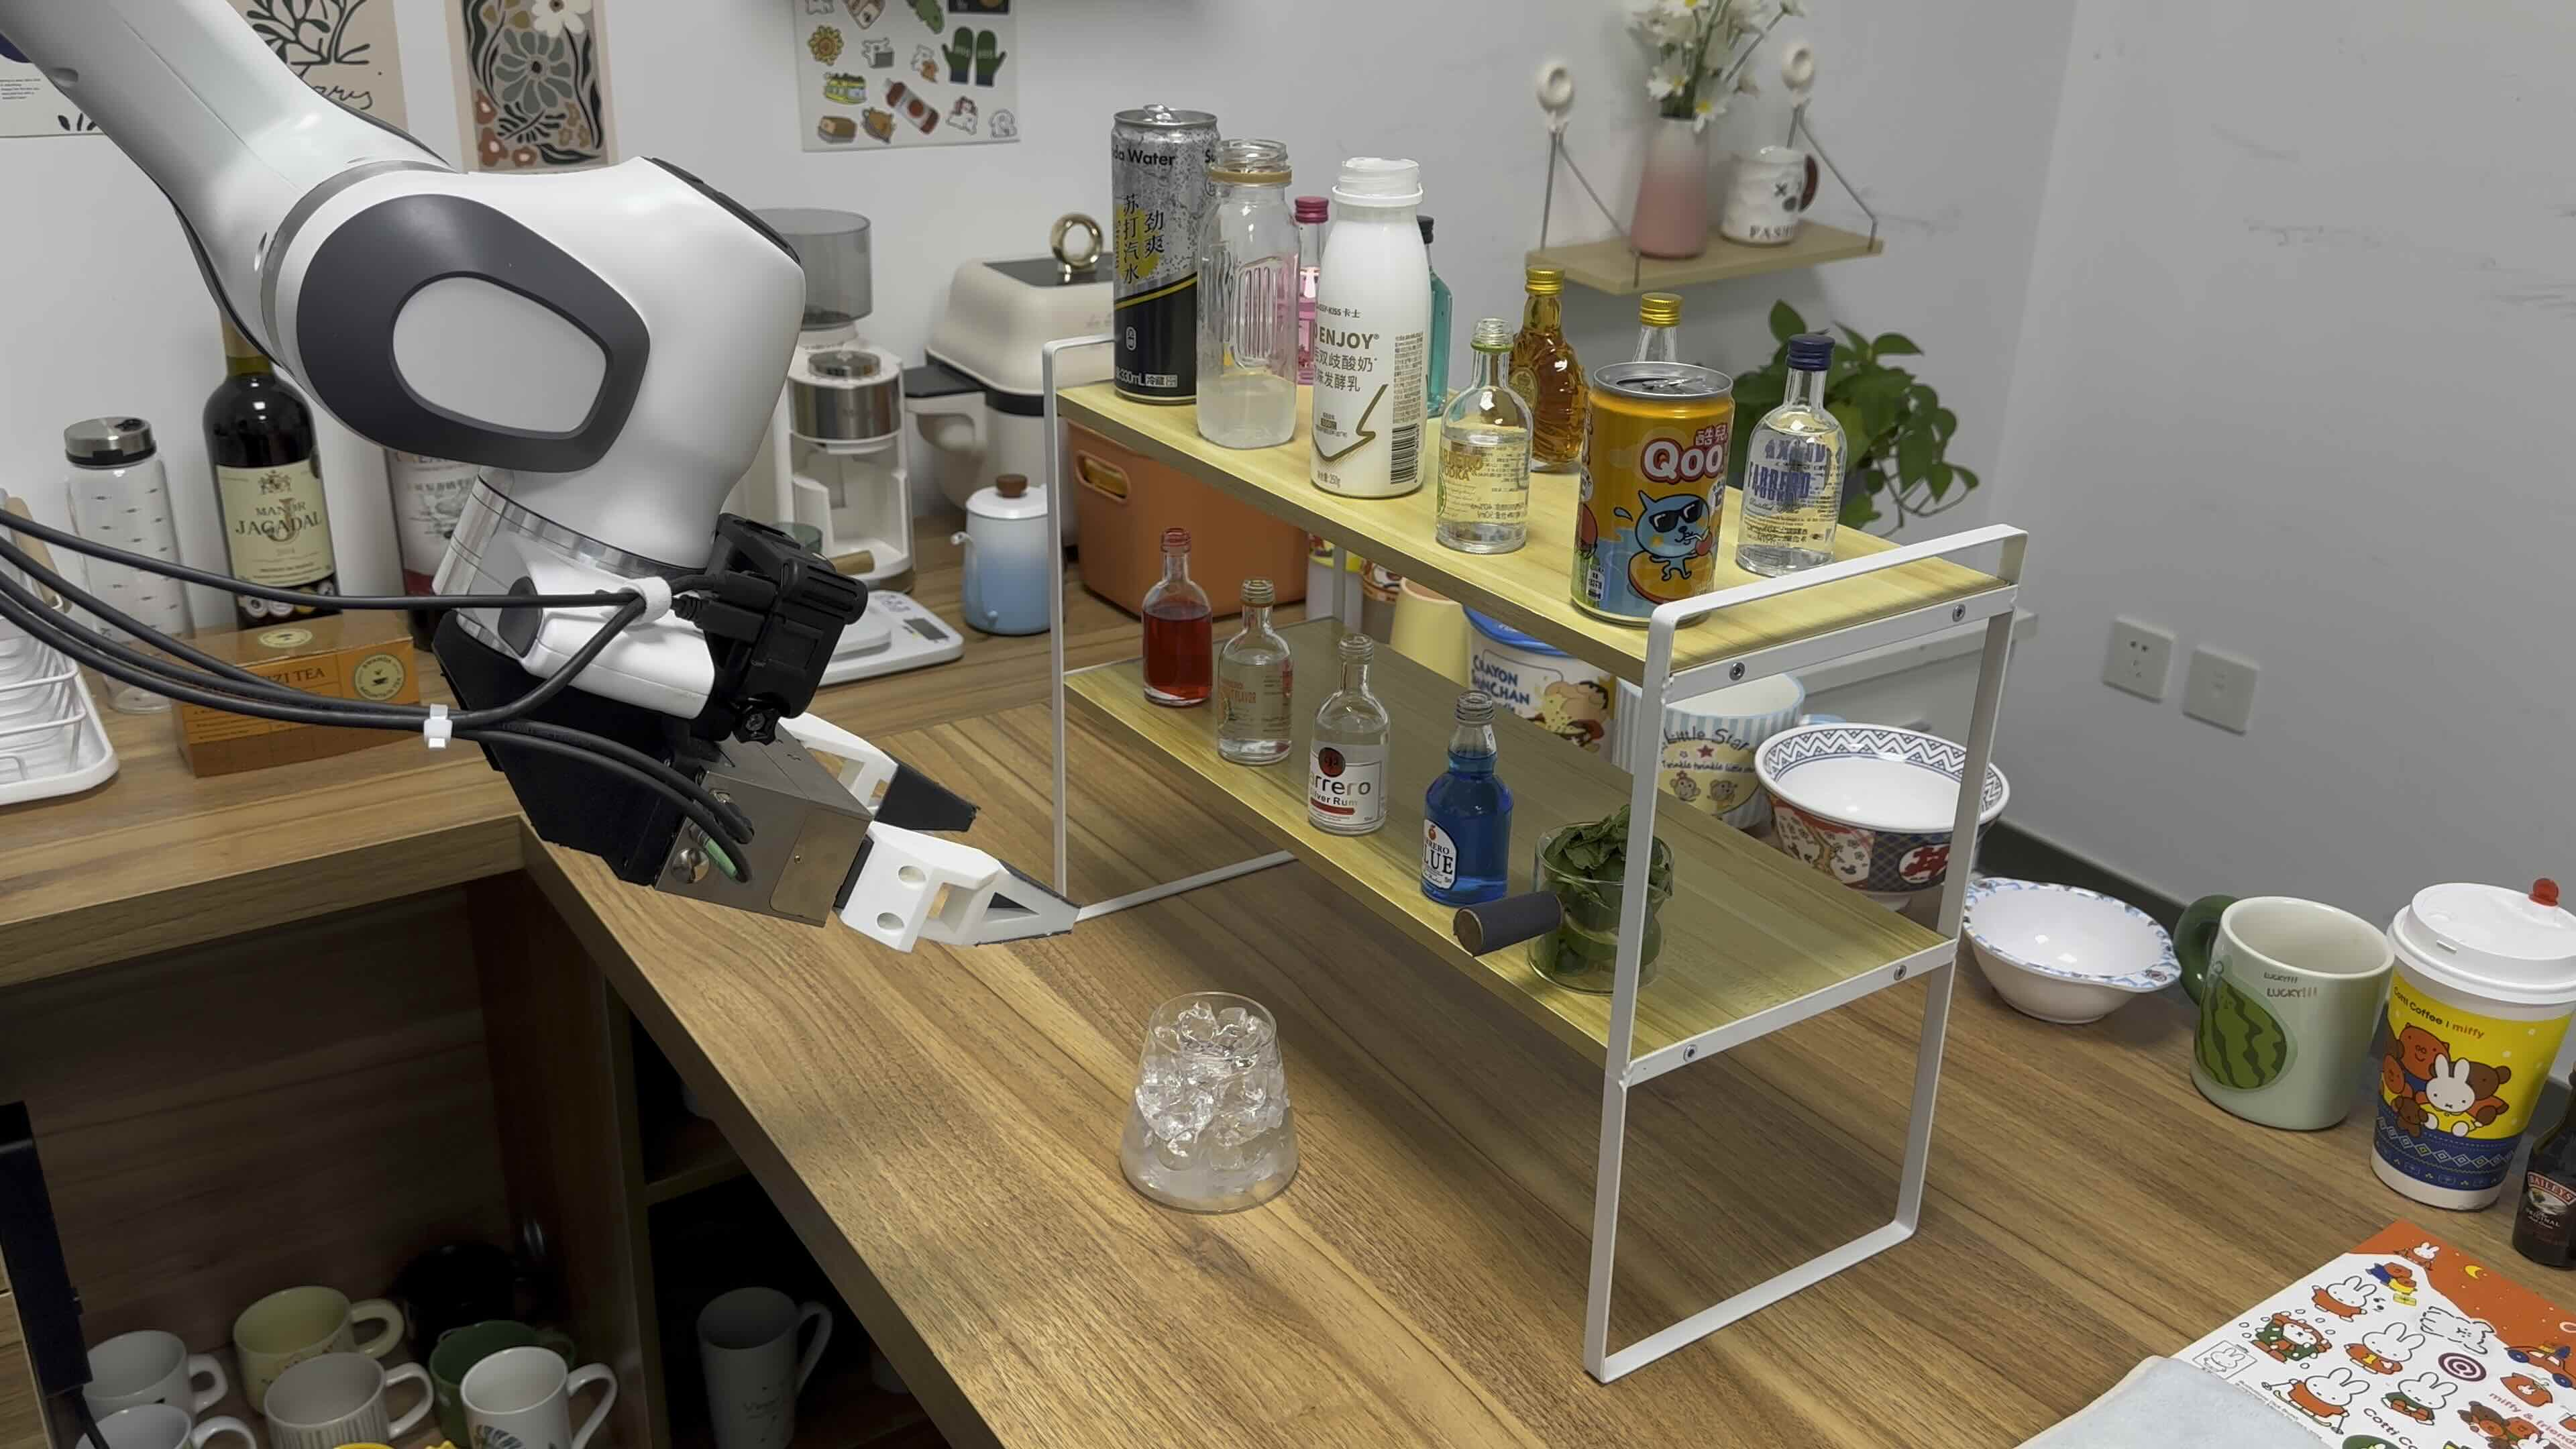}}
        & % Column separator
        \begin{minipage}[\imagevalign]{\colCwidth}
            \raggedright
            \textbf{Instruction}: Make me a cup of \texttt{Mountain Fuji} cocktail. \\
            \textbf{Reasoning}:\\
            \textsf{Scene description}: The orange-flavored vodka is the second from the left on the bottom shelf. The Blue Curacao is the second from the right on the bottom shelf. The lemon juice is the second from the left on the top shelf. The yogurt is located in the middle of the top shelf.  \\
            \textsf{Plan}:  1. Pour the orange-flavored vodka into the glass. 2. Pour the Blue Curacao into the glass. 3. Pour the lemon juice into the glass. 4. Pour the yogurt into the glass. \\
            \textsf{What I have done}: Nothing.\\
            \textsf{Now I need to}: Pour the orange-flavored vodka into the glass.
        \end{minipage} \\ % End of table row
        \bottomrule % Bottom rule line
    \end{tabular}
    \vspace{2pt}
    \caption{\textbf{Reasoning examples for long-horizon task planning.}}
    \label{tab:plan_reasoning_eg}
\end{table}
