# Supplementary material for: ReFineVLA: Multimodal Reasoning-Aware Generalist Robotic Policies via Teacher-Guided Fine-Tuning
Source: arXiv:2604.17800 source file (2026-04-20)
Supplement: Supplementary file 6 [file table.tex]

% Set the column widths as fractions of \linewidth
% Adjust these fractions as needed.
% Ensure the sum of fractions is slightly less than 1.0 to leave space for \tabcolsep.
\setlength{\colAwidth}{0.25\linewidth}
\setlength{\colBwidth}{0.1\linewidth}
\setlength{\colCwidth}{0.7\linewidth}
\setlength{\figurewidth}{\colAwidth}

\begin{table}[H]
    \centering
    \small % Use smaller font size

    % Define the table structure:
    % Column 1: aligned center for images using \adjustbox
    % Column 2: aligned left, controlled by \minipage for captions
    \begin{tabular}{ll}
        \toprule % Top rule line

        % --- First Row: Direct mouse ---
        % Image: Use adjustbox to align the top
        \adjustbox{valign=t}{\includegraphics[width=\figurewidth]{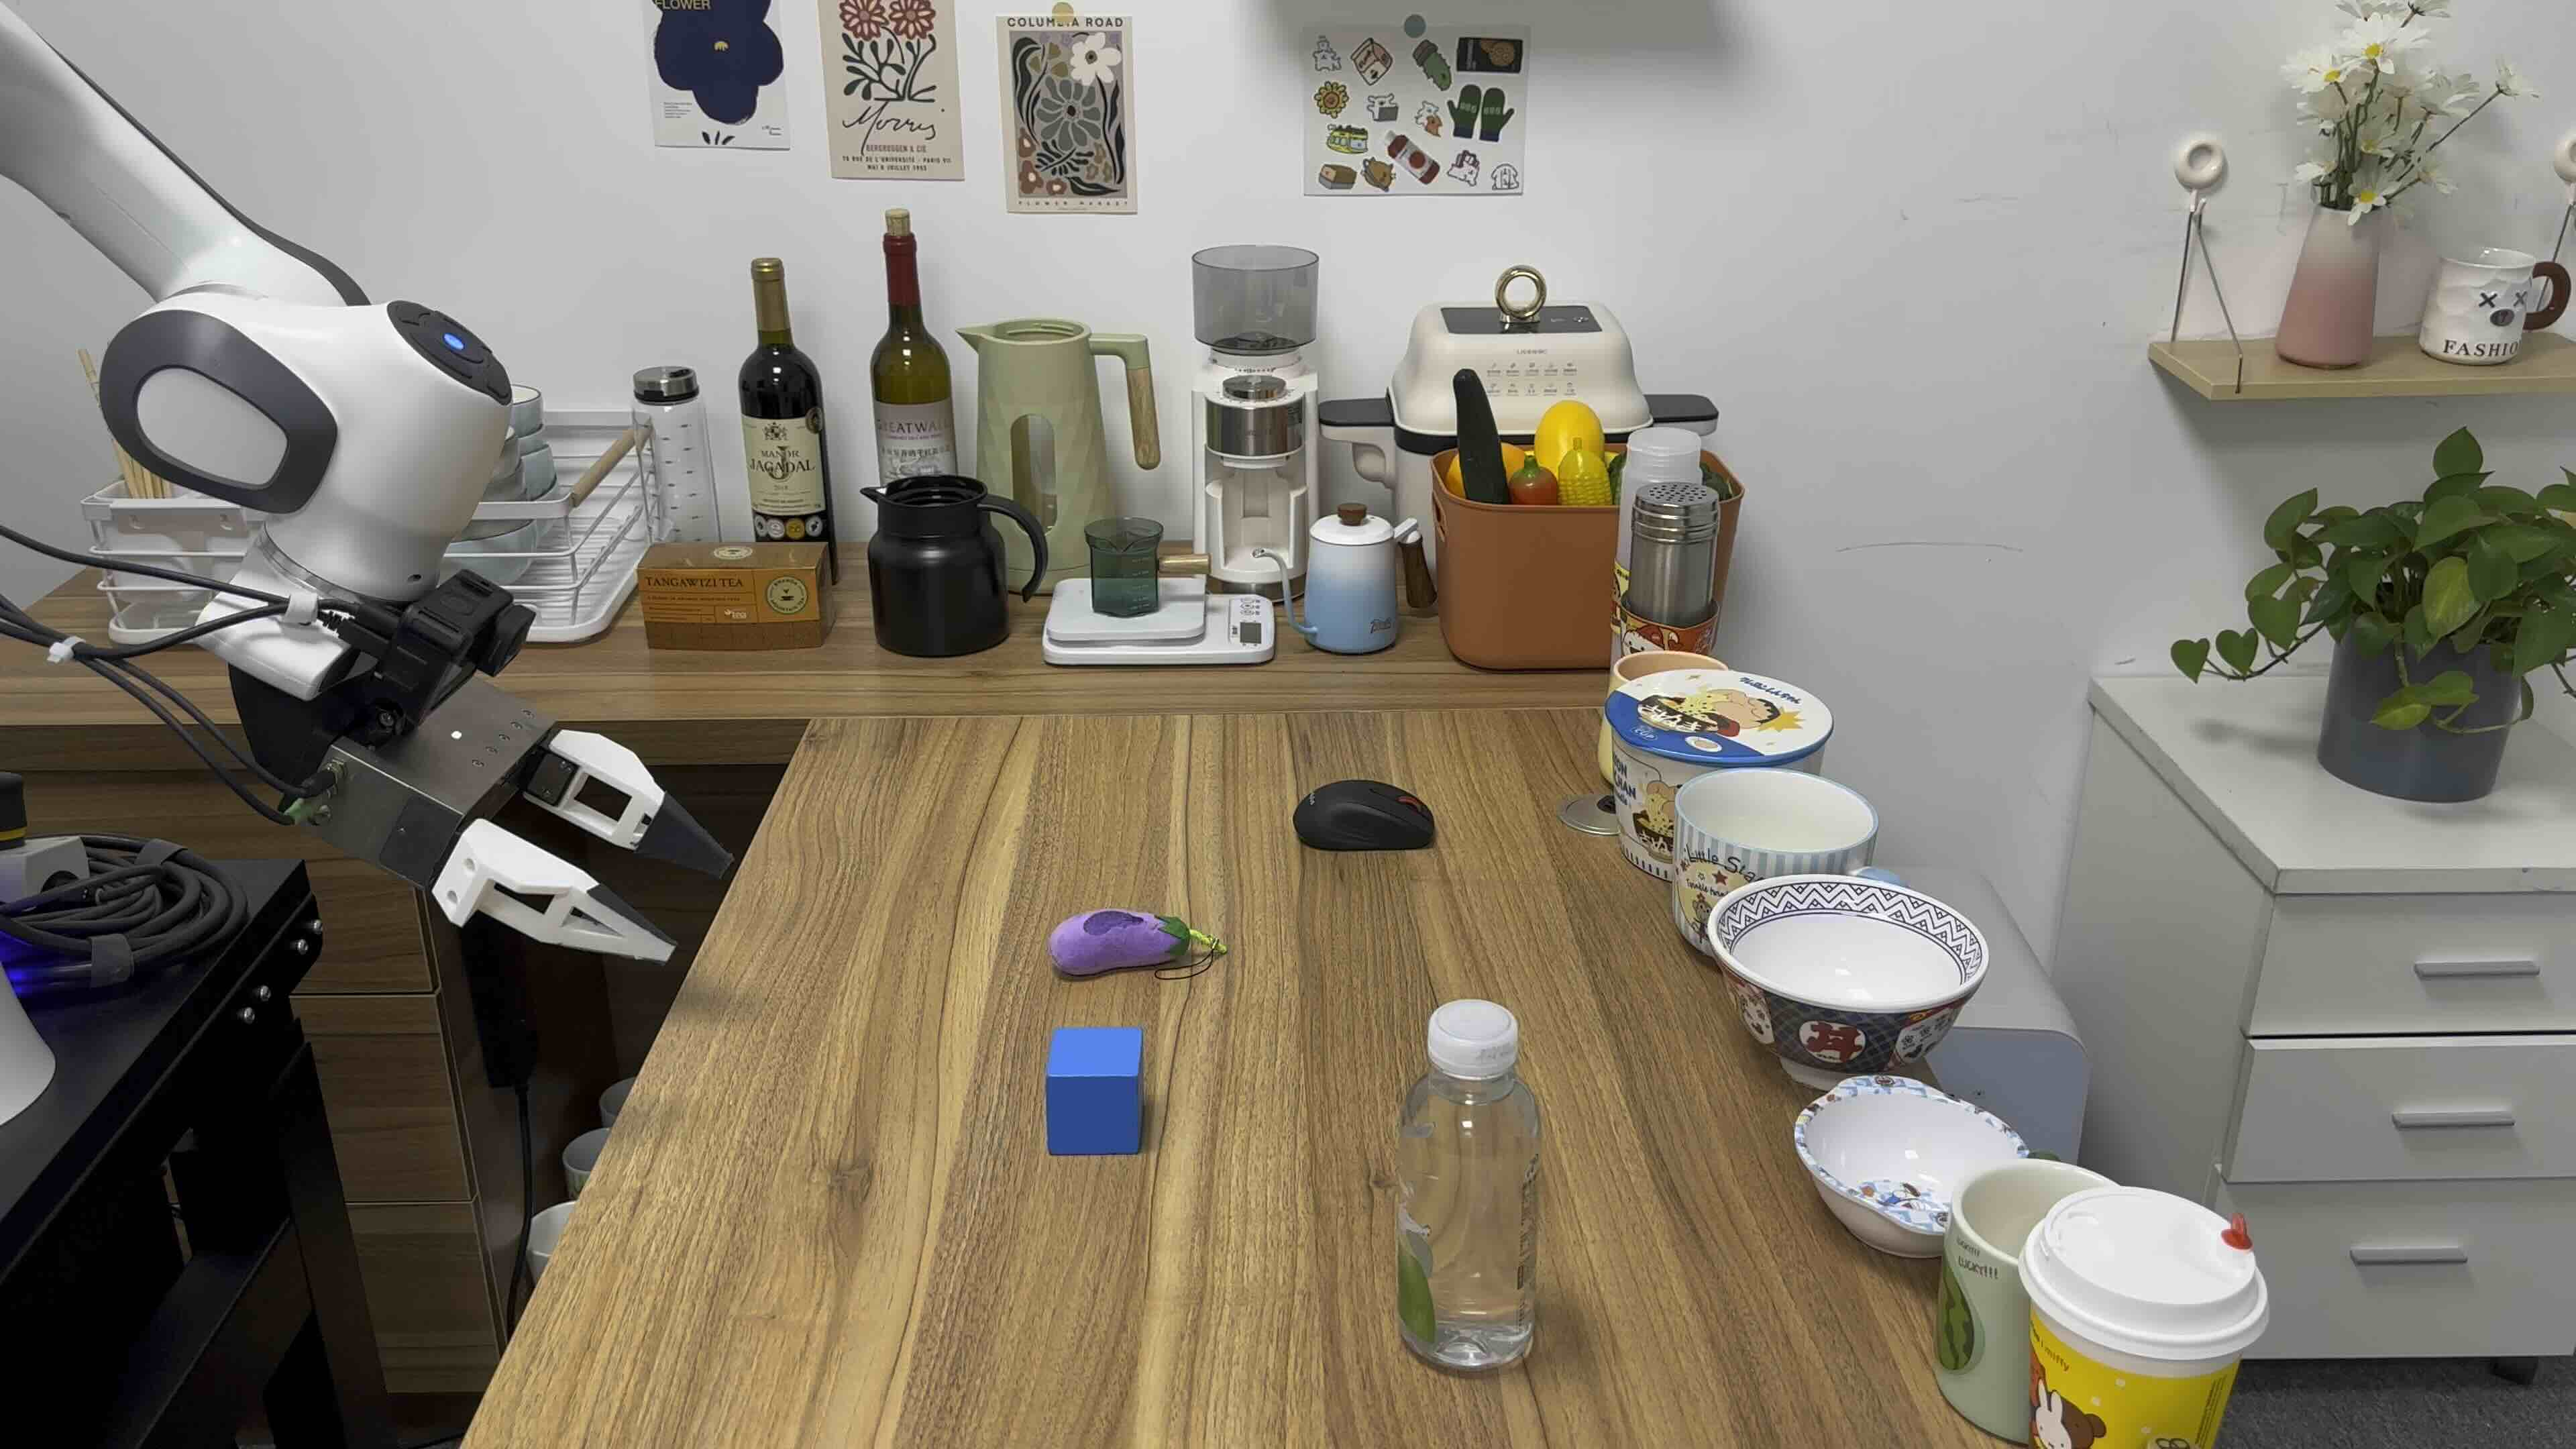}}
        & % Column separator
        % Caption: Place all text in a minipage, use [t] for top alignment
        \begin{minipage}[t]{\colCwidth}
            \raggedright % Recommended in narrow columns to avoid excessive spacing
            \textbf{Instruction}: Pick up the black mouse. \\
            \textbf{Reasoning}:\\
            I need to pick up the black mouse, which is to the left back of the eggplant, has a smooth, arching shape that fits the palm, and is a key component of a typical office workstation.
        \end{minipage} \\ % End of table row
        \midrule % Mid rule line

        % --- Second Row: Spatial Cube ---
        \adjustbox{valign=t}{\includegraphics[width=\figurewidth]{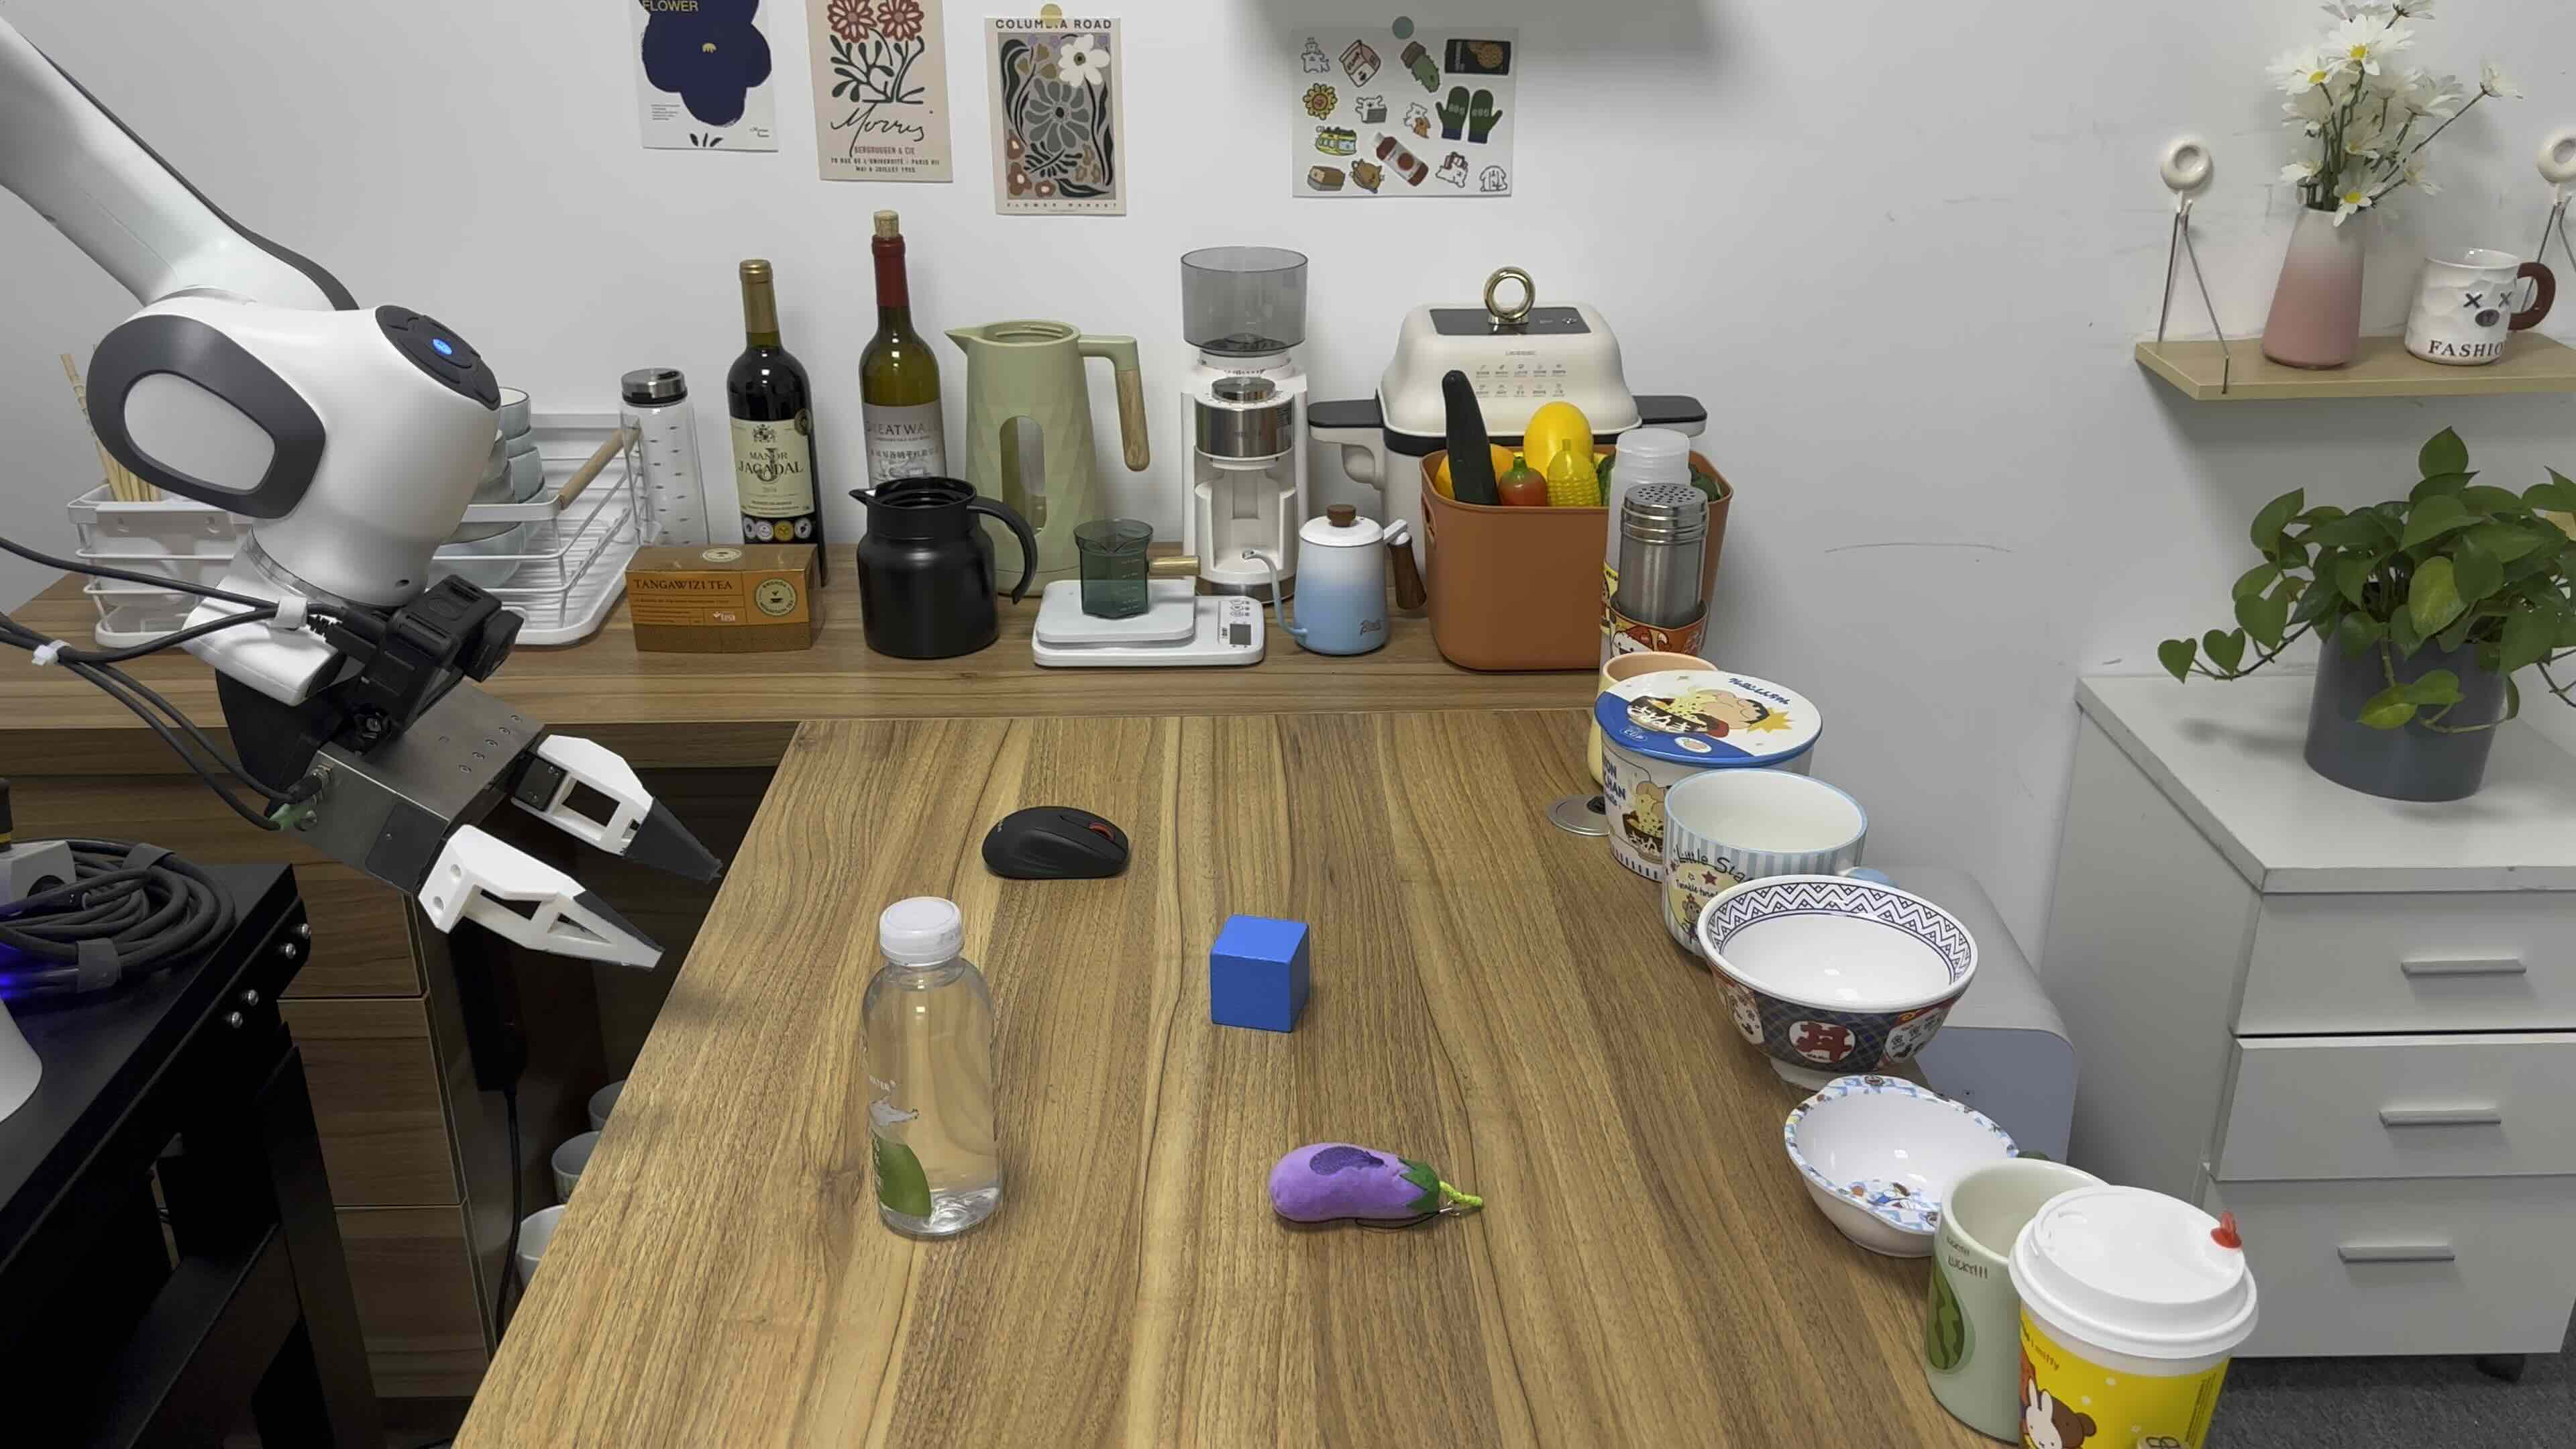}}
        & % Column separator
        \begin{minipage}[t]{\colCwidth}
            \raggedright
            \textbf{Instruction}: Pick up the object which is to the left back of the coconut water bottle. \\
            \textbf{Reasoning}: \\
            I need to pick up the blue cube, which is identified by its blue shade, and is a solid form useful for creating stable structures. \\
        \end{minipage} \\ % End of table row
        \midrule % Mid rule line

        % --- Third Row: Attribute Eggplant ---
        \adjustbox{valign=t}{\includegraphics[width=\figurewidth]{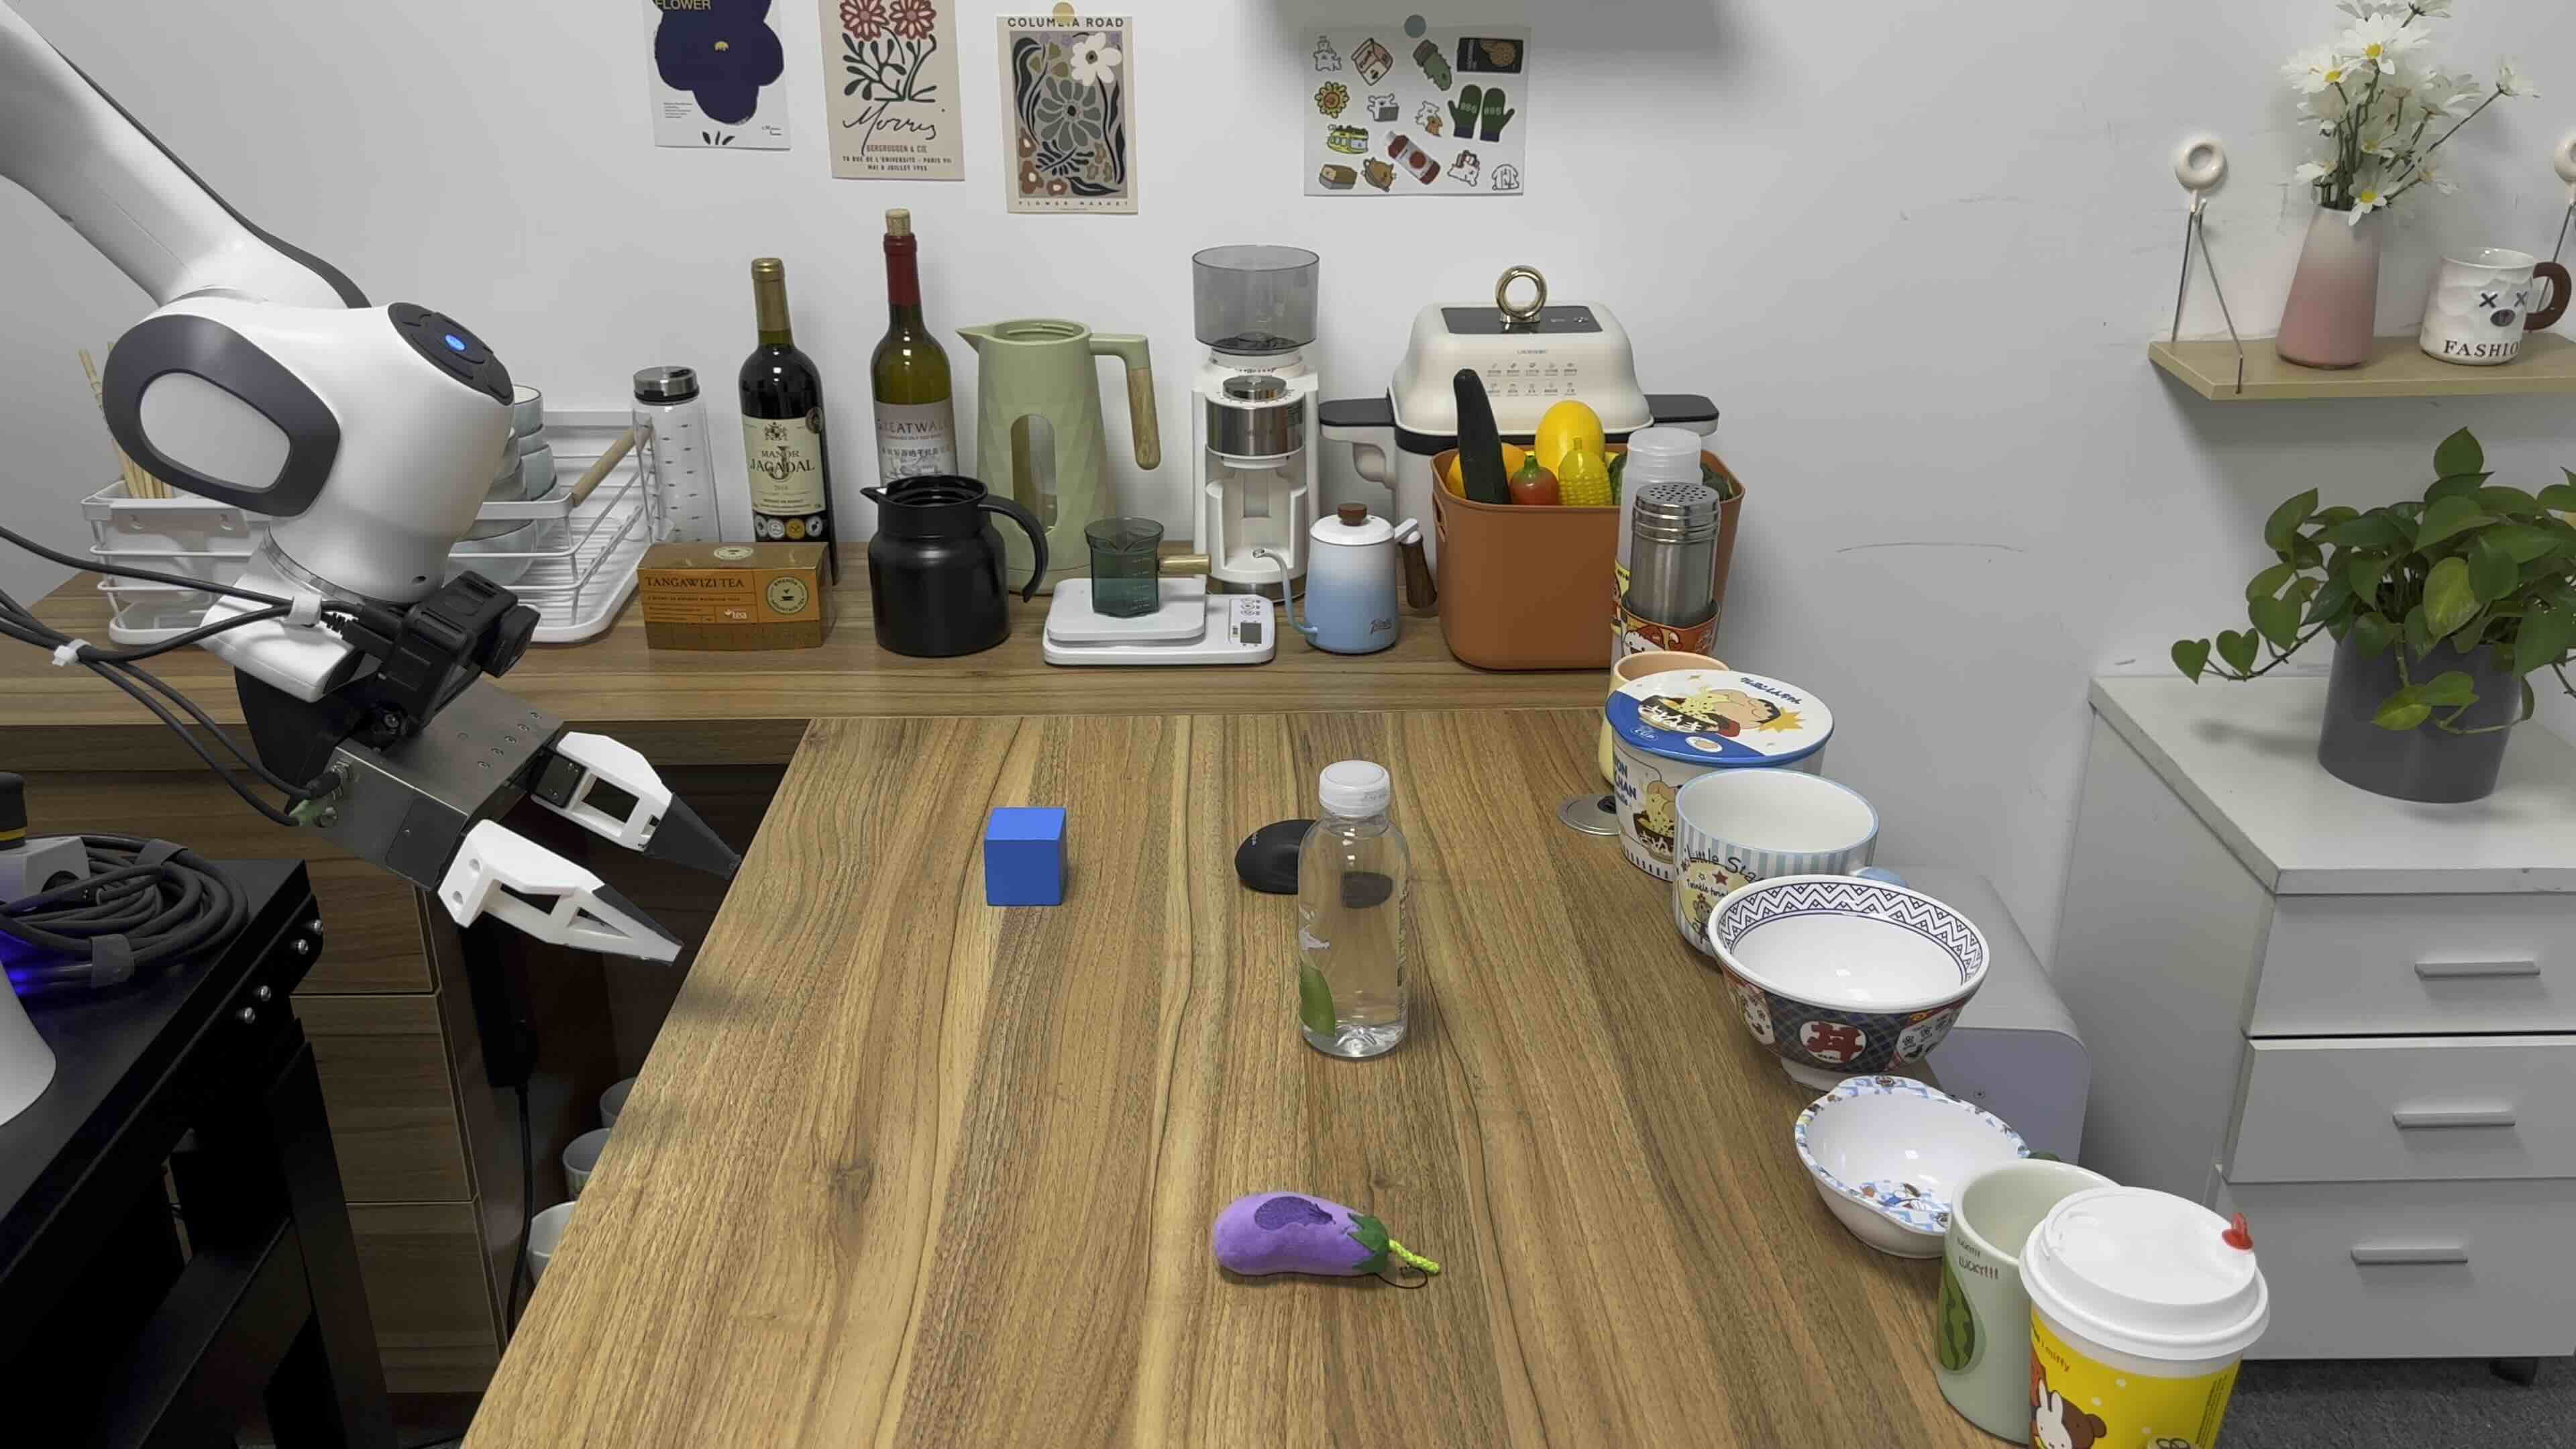}}
        & % Column separator
        \begin{minipage}[t]{\colCwidth}
            \raggedright
            \textbf{Instruction}: Pick up the object which exhibits a purple coloration. \\
            \textbf{Reasoning}: \\
            I need to pick up the eggplant, which is to the right of the coconut water bottle, and is a common ingredient in ratatouille. \\
        \end{minipage} \\ % End of table row
        \midrule

        % --- Fourth Row: Semantic Coconut Water ---
        \adjustbox{valign=t}{\includegraphics[width=\figurewidth]{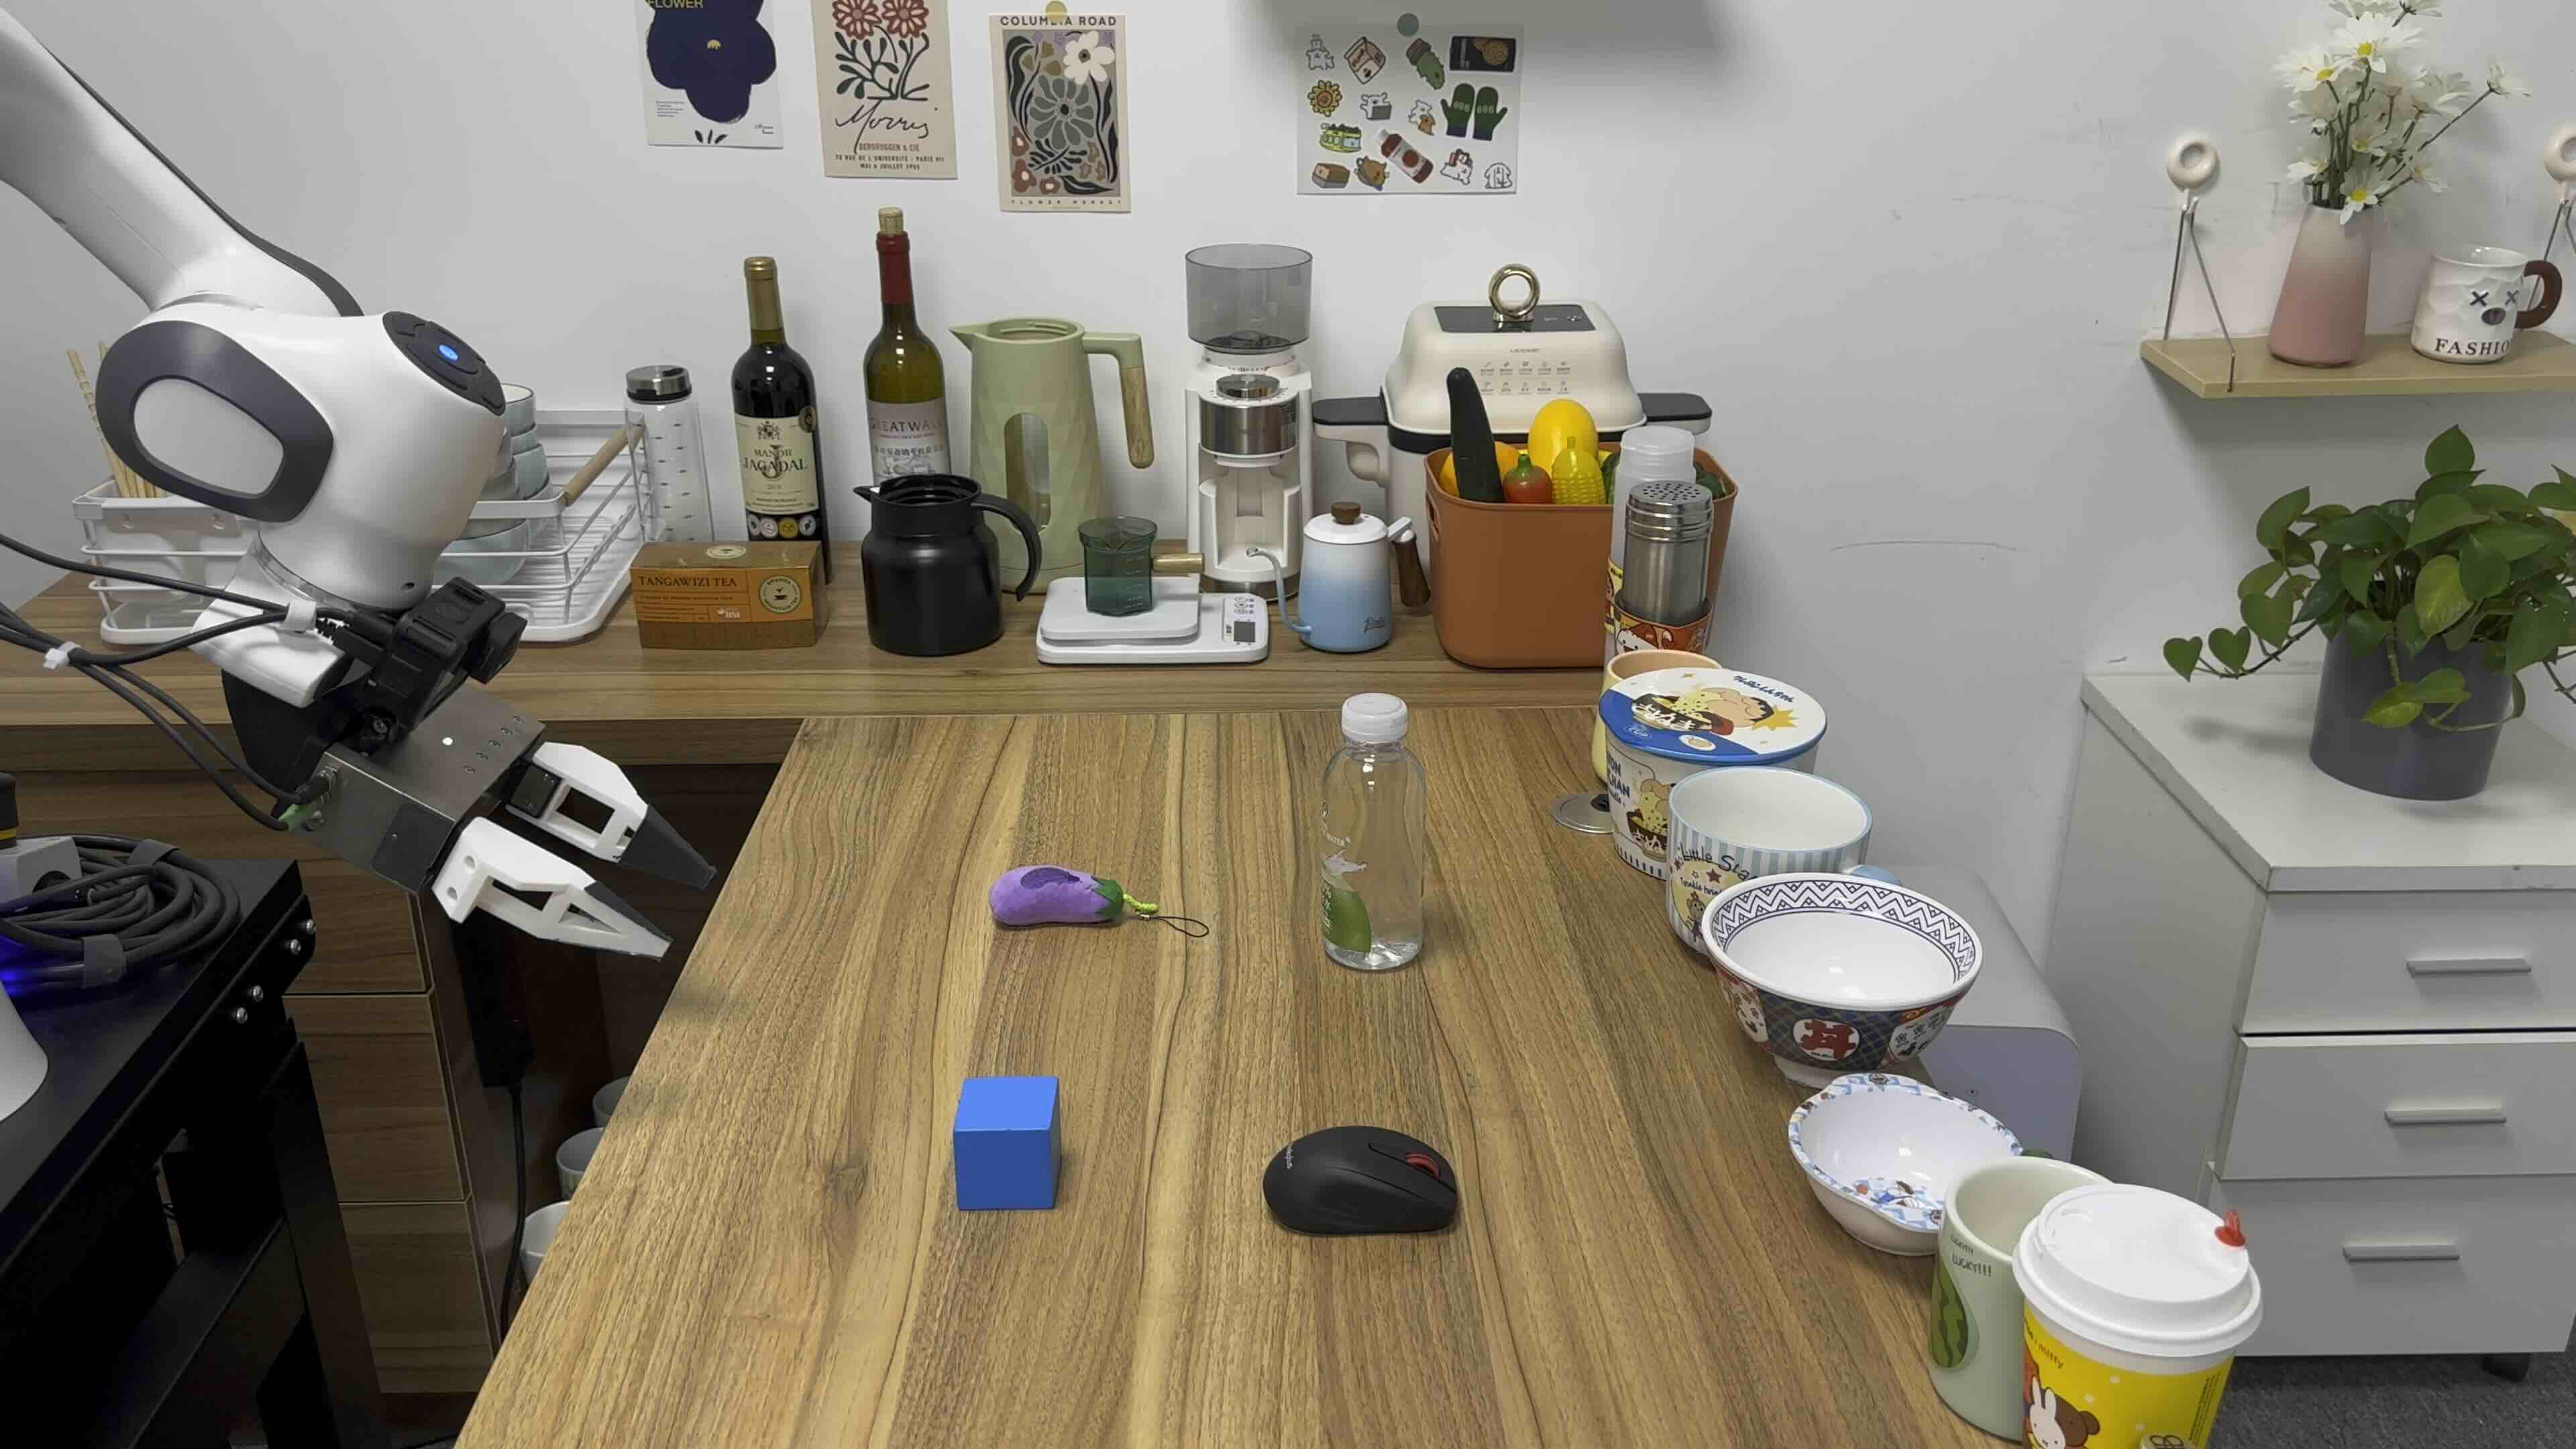}}
        & % Column separator
        \begin{minipage}[t]{\colCwidth}
            \raggedright
            \textbf{Instruction}: Pick up the object which is a packaged drink. \\
            \textbf{Reasoning}: \\
            I need to pick up the coconut water bottle, which is to the left back of the blue cube, and has a cylindrical form. \\
        \end{minipage} \\ % End of table row

        \bottomrule % Bottom rule line
    \end{tabular}
    \vspace{2pt}
    \caption{\textbf{Reasoning examples for \texttt{Single-Env} visual grounding.}}
    \label{tab:single_env_visual_grounding_reasoning_eg}
\end{table}
