# Supplementary material for: ReFineVLA: Multimodal Reasoning-Aware Generalist Robotic Policies via Teacher-Guided Fine-Tuning
Source: arXiv:2604.17800 source file (2026-04-20)
Supplement: Supplementary file 8 [file table.tex]

% Set the column widths as fractions of \linewidth
% Adjust these fractions as needed.
% Ensure the sum of fractions is slightly less than 1.0 to leave space for \tabcolsep.
\setlength{\colAwidth}{0.25\linewidth}
\setlength{\colBwidth}{0.1\linewidth}
\setlength{\colCwidth}{0.7\linewidth}
\setlength{\figurewidth}{\colAwidth}

\begin{table}[H] % Use htbp for more placement options
    \centering
    \small % Use smaller font size

    % Define the table structure:
    % Column 1: aligned center for images using \adjustbox
    % Column 2: aligned left, controlled by \minipage for captions
    \begin{tabular}{ll}
        \toprule % Top rule line

        % --- First Row: Hotpot ---
        % Image: Use adjustbox to align the top
        \adjustbox{valign=\imagevalign}{\includegraphics[width=\figurewidth]{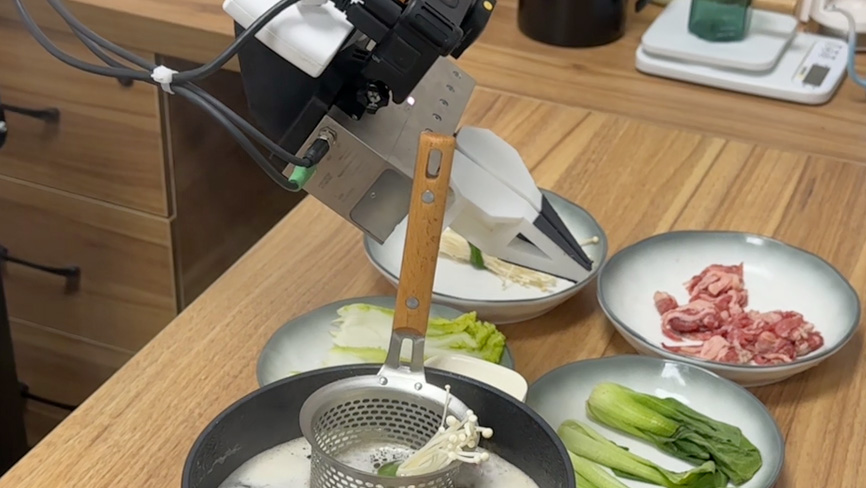}}
        & % Column separator
        \begin{minipage}[\imagevalign]{\colCwidth}
            \raggedright % Recommended in narrow columns to avoid excessive spacing
            \textbf{Instruction}: Dip the beef and the enoki mushrooms. \\
            \textbf{Reasoning}:\\
            \textsf{Scene description}: Some of the beef and the green bok choy are in the hotpot strainer. \textit{But I fail to grasp the hotpot strainer due to misalignment.} \\
            \textsf{Plan}: 1. Put the beef into the hotpot strainer. 2. Put the enoki mushrooms into the hotpot strainer. 3. Wait for the ingredients to cook and then pick up the hotpot strainer. \\
            \textsf{What I have done}: 1. Put the beef into the hotpot strainer. 2. Put the enoki mushrooms into the hotpot strainer. \\
            \textsf{Now I need to}: \textit{Retract, reposition to align with the strainer, and try grasping again.}
        \end{minipage} \\ % End of table row
        \midrule % Mid rule line

        % --- Second Row: Tomato ---
        \adjustbox{valign=\imagevalign}{\includegraphics[width=\figurewidth]{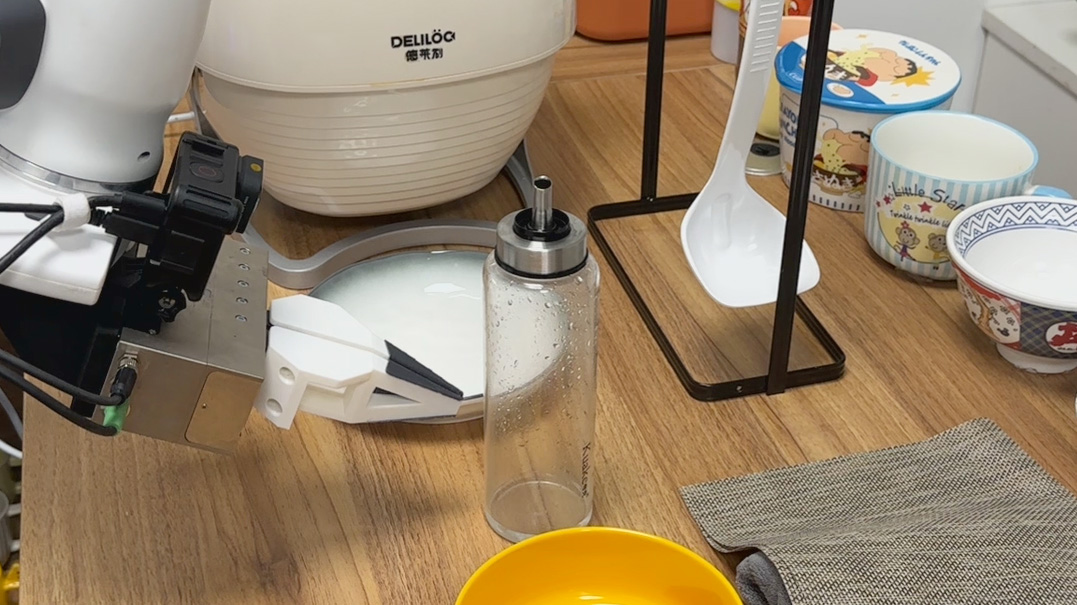}}
        & % Column separator
        \begin{minipage}[\imagevalign]{\colCwidth}
            \raggedright
            \textbf{Instruction}: Make me a plate of tomato-egg scramble. \\
            \textbf{Reasoning}:\\
            \textsf{Scene description}: The oil bottle is located at the front of the table. The cooking machine is on the left side of the table. \textit{But I discover that the oil bottle slips from the gripper.} \\
            \textsf{Plan}:  1. Pour the oil into the cooking machine. 2. Pour the tomatoes and egg liquid into the cooking machine. 3. Wait for the cooking process to finish, then pick up the spoon. 4. Scoop out the tomato-egg scramble, transfer it onto the plate, and place the spoon into the cooking machine. \\
            \textsf{What I have done}: Nothing.\\
            \textsf{Now I need to}: \textit{Retry to grasp the oil bottle with increased firmness.}
        \end{minipage} \\ % End of table row

        \bottomrule % Bottom rule line
    \end{tabular}
    \vspace{2pt}
    \caption{\textbf{Reasoning examples for error detection and recovery.}}
    \label{tab:error_reasoning_eg}
\end{table}
